# Supplementary material for: DPOK: Reinforcement Learning for Fine-tuning Text-to-Image Diffusion Models
Source: arXiv:2305.16381 source file (2023-11-01)
Supplement: Supplementary file 1 [file appendix.tex]

\appendix

\begin{center}{\bf {\LARGE Appendix:}}
\end{center}
\begin{center}{\bf {\Large Reinforcement Learning for \\ Fine-tuning Text-to-Image Diffusion Models}}
\end{center}

\section{Derivations}
\subsection{Lemma~\ref{lemma_pg}}
\label{proof_pg}

\begin{proof}
    
\begin{align*}
&\mathrel{\phantom{=}}\nabla_{\theta} \mathbb{E}_{p(z)}\mathbb{E}_{p_\theta(x_0|z)}\left[-r(x_0,z)\right] = -\mathbb{E}_{p(z)}\left[\nabla_{\theta}\int p_\theta(x_0|z)r(x_0,z) dx_0\right] \\ 
&=-\mathbb{E}_{p(z)}\left[\nabla_{\theta}\int \left(\int p_\theta(x_{0:T}|z) dx_{1:T}\right)r(x_0,z) dx_0\right] \\ 
&= -\mathbb{E}_{p(z)}\left[\int \nabla_{\theta}\log p_\theta(x_{0:T}|z) \times r(x_0,z) \times p_\theta(x_{0:T}|z) \; dx_{0:T}\right] \\
&= -\mathbb{E}_{p(z)}\left[\int \nabla_{\theta}\log\left(p_T(x_T|z)\prod_{t=1}^Tp_\theta(x_{t-1}|x_t,z)\right) \times r(x_0,z) \times p_\theta(x_{0:T}|z) \; dx_{0:T}\right] \\
&=-\mathbb{E}_{p(z)}{\mathbb{E}_{p_\theta(x_{0:T}|z)}}\left[r(x_0,z) \sum_{t=1}^{T} \nabla_{\theta}\log p_{\theta}(x_{t-1}|x_{t},z)\right],
\end{align*}
where the second last equality is from the continuous assumptions of $p_\theta(x_{0:T}|z)r(x_0,z)$ and $\nabla_{\theta}p_\theta(x_{0:T}|z)r(x_0,z)$.
\end{proof}

\subsection{Lemma~\ref{lemma_online_kl}}
\label{app: online_kl}

Similar to the proof in Theorem 1 in~\cite{song2021maximum}, from data processing inequality with the Markov kernel, given any $z$ we have

\begin{equation}
    \text{KL}(p_\theta (x_0|z)) \|p_{\text{pre}}(x_0|z)) \leq\text{KL}(p_\theta(x_{0:T}|z) \| p_{\text{pre}}(x_{0:T}|z)).
\end{equation}

Using the Markov property of $p_\theta$ and $p_{\text{pre}}$, we have
\begin{align*}
&\mathrel{\phantom{=}}\text{KL}(p_\theta(x_{0:T}|z) \| p_{\text{pre}}(x_{0:T}|z)) = \int p_\theta(x_{0:T}|z) \times \log \frac{p_\theta(x_{0:T}|z)}{p_{\text{pre}}(x_{0:T}|z)} \; d x_{0:T}\\
&= \int p_\theta(x_{0:T}|z) \log \frac{p_\theta(x_T|z) \prod_{t=1}^T p_\theta(x_{t-1} |x_t,z)}{p_{\text{pre}}(x_T|z) \prod_{t=1}^T p_{\text{pre}}(x_{t-1} | x_t,z)} dx_{0:T} \\
&= \int p_\theta(x_{0:T}|z) \left(\log\frac{p_\theta(x_T|z)}{p_{\text{pre}}(x_T|z)} + \sum_{t=1}^T \log \frac{p_\theta(x_{t-1} | x_t,z)}{p_{\text{pre}}(x_{t-1} | x_t,z)}\right) d x_{0:T} \\
&= \mathbb{E}_{p_\theta(x_{0:T}|z)}\left[\sum_{t=1}^T\log \frac{p_\theta(x_{t-1}|x_t,z)}{p_{\text{pre}}(x_{t-1}|x_t,z)}\right] = \sum_{t=1}^{T}\mathbb{E}_{p_\theta(x_{t:T}|z)}\mathbb{E}_{p_\theta(x_{0:t-1}|x_{t:T},z)}\left[\log \frac{p_\theta(x_{t-1}|x_t,z)}{p_{\text{pre}}(x_{t-1}|x_t,z)}\right] \\
& =\sum_{t=1}^{T}\mathbb{E}_{p_\theta(x_{t}|z)}\mathbb{E}_{p_\theta(x_{0:t-1}|x_{t},z)}\left[\log \frac{p_\theta(x_{t-1}|x_t,z)}{p_{\text{pre}}(x_{t-1}|x_t,z)}\right] = \sum_{t=1}^{T}\mathbb{E}_{p_\theta(x_{t}|z)}\mathbb{E}_{p_\theta(x_{t-1}|x_{t},z)}\left[\log \frac{p_\theta(x_{t-1}|x_t,z)}{p_{\text{pre}}(x_{t-1}|x_t,z)}\right] \\
&= \sum_{t=1}^{T}\mathbb{E}_{p_\theta(x_{t}|z)}\big[\text{KL}\big(p_\theta(x_{t-1}|x_t,z) \| p_{\text{pre}}(x_{t-1}|x_t, z)\big)\big].
\end{align*}

Taking the expectation of $p(z)$ on both sides, we have 
% \ow{Where does the inequality come from?} -> see the first inequality in this proof

\begin{equation}
\mathbb{E}_{p(z)}[\text{KL}(p_\theta (x_0|z)) \|p_{\text{pre}}(x_0|z))] \leq \mathbb{E}_{p(z)}\left[\sum_{t=1}^{T}\mathbb{E}_{p_\theta(x_{t}|z)}\big[\text{KL}\big(p_\theta(x_{t-1}|x_t,z) \| p_{\text{pre}}(x_{t-1}|x_t, z)\big)\big]\right].
\end{equation}

\subsection{The objective in eq.~(\ref{eq:online})}
\label{app: partial_gradient}
From Lemma~\ref{lemma_online_kl}, for online fine-tuning, at each step $t\leq T$, we need to regularize $\sum_{t=1}^T\mathbb{E}_{p_\theta(x_t)}\big[\text{KL}\big(p_\theta(x_{t-1}|x_t,z)\| p_{\text{pre}}(x_{t-1}|x_t, z)\big)\big]$.
% given any $z$. Note that from 
By the product rule, we have
\begin{align}
\label{partial_grad}
&\sum_{t=1}^T\nabla_\theta\mathbb{E}_{p_\theta(x_t)}\big[\text{KL}\big(p_\theta(x_{t-1}|x_t,z) \| p_{\text{pre}}(x_{t-1}|x_t, z)\big)\big] \nonumber \\
&\quad= \sum_{t=1}^T\mathbb{E}_{p_\theta(x_t)}\big[\nabla_\theta \text{KL}\big(p_\theta(x_{t-1}|x_t,z) \| p_{\text{pre}}(x_{t-1}|x_t, z)\big)\big] \\ 
&\quad+\sum_{t=1}^T\mathbb{E}_{p_\theta(x_t)}\big[\nabla_\theta \log p_\theta(x_t)\cdot\text{KL}\big(p_\theta(x_{t-1}|x_t,z) \| p_{\text{pre}}(x_{t-1}|x_t, z)\big)\big]. \nonumber
\end{align}
Moreover, the second term in Eq.~(\ref{partial_grad}) can be rewritten as
\begin{equation}
\begin{aligned}
&\sum_{t=1}^T\mathbb{E}_{p_\theta(x_t)}\big[\nabla_\theta \log p_\theta(x_t) \cdot \text{KL}\big(p_\theta(x_{t-1}|x_t,z) \| p_{\text{pre}}(x_{t-1}|x_t, z)\big)\big] \\
& \quad= \sum_{t=1}^T\mathbb{E}_{p_\theta(x_t)}\big[\sum_{t'>t}^T \nabla_\theta \log p_\theta(x_{t'-1}|x_{t'}, z) \cdot \text{KL}\big(p_\theta(x_{t-1}|x_t,z) \| p_{\text{pre}}(x_{t-1}|x_t, z)\big)\big], 
\end{aligned}   
\end{equation}
which treats the sum of conditional KL-divergences along the prior sub-trajectory as a scalar reward at each step. However, computing these sums is more inefficient than just the first term in Eq.~(\ref{partial_grad}). Empirically, we find that regularizing only the first term in Eq.~(\ref{partial_grad}) works well, 
% so we adopt the first term in Eq.~(\ref{partial_grad}) when calculating the gradient for simplicity, 
so we adopt this approach for simplicity, which yields the KL-regularized objective in eq.~(\ref{eq:online}).

\subsection{Lemma~\ref{lemma_sup_kl}}
\label{proof_sup_kl}
Similar to derivation in~\cite{ho2020denoising}, and notice that $q$ is not dependent on $z$ (i.e., $q(\dotsb|z) = q(\dotsb)$), we have

\begin{equation}
\begin{aligned}
&\mathrel{\phantom{=}}\mathbb{E}_{p(z)}\mathbb{E}_{p_{\text{pre}}(x_0|z)}[-(r(x_0,z)+\gamma)\log{p_\theta(x_0|z)}] \\
% & =\mathbb{E}_{p(z)}\mathbb{E}_{p_{\text{pre}}(x_0|z)}\mathbb{E}_{p_{\text{pre}}(x_{1:T}|x_0, z)}[-\log{p_\theta(x_0|z)}] \\
&\leq\mathbb{E}_{p(z)}\mathbb{E}_{p_\text{pre}(x_0|z)}\mathbb{E}_{q(x_{1:T}|x_0, z)}[-(r(x_0,z)+\gamma)\log\frac{p_\theta(x_{0:T}|z)}{q(x_{1:T}|x_0, z)}]\\
&=
\mathbb{E}_{p(z)}\mathbb{E}_{p_\text{pre}(x_0|z)}\mathbb{E}_{q(x_{1:T}|x_0, z)}[-(r(x_0,z)+\gamma)\log \frac{p(x_T|z)}{q(x_T|x_0, z)}\\
&\mathrel{\phantom{=}}-\sum_{t>1}(r(x_0,z)+\gamma)\log 
\frac{p_\theta(x_{t-1}|x_t,z)}{q(x_{t-1}| x_t, x_0,z)}\\
&\mathrel{\phantom{=}}-(r(x_0,z)+\gamma)\log p_{\theta}(x_0|x_1, z)]\\
& = \mathbb{E}_{p(z)}\mathbb{E}_{p_\text{pre}(x_0|z)}[(r(x_0,z)+\gamma)\mathbb{E}_{q(x_T|x_0, z)}[\text{KL}(q(x_T|x_0) \|p(x_T))] \\
&\mathrel{\phantom{=}}+(r(x_0,z)+\gamma)\sum_{t>1} \mathbb{E}_{q(x_t|x_0, z)}[\text{KL}(q(x_{t-1}|x_t, x_0) \| p_\theta(x_{t-1}|x_t, z))] \\
&\mathrel{\phantom{=}}-(r(x_0,z)+\gamma)\mathbb{E}_{q(x_1|x_0, z)}[\log p_{\theta}(x_0|x_1, z)]],\\
\end{aligned}
\end{equation}
where the first inequality comes from ELBO.
Let $f_{\theta}(x_t, t, z) := (x_t - \sqrt{1 -\alpha_t} \epsilon_{\theta}(x_t, t, z))/\sqrt{\alpha_t}$, $\sigma_t^2 := \frac{1-\bar{\alpha}_{t-1}}{1-\bar{\alpha}_t}\beta_t$. Optimizing the above bound is equivalent to optimizing 
\begin{equation}
\begin{aligned}
\label{tighter_bound}
&\mathrel{\phantom{=}}\mathbb{E}_{p(z)}\mathbb{E}_{p_\text{pre}(x_0|z)}[(r(x_0,z)+\gamma)\mathbb{E}_{q(x_T|x_0, z)}[\text{KL}(q(x_T|x_0) \|p(x_T))]\\
&\mathrel{\phantom{=}}+(r(x_0,z)+\gamma)\sum_{t>1} \mathbb{E}_{q(x_t|x_0, z)}[\frac{||x_0 - f_\theta(x_t, t, z)||^2}{2\sigma_t^2}] \\
&-(r(x_0,z)+\gamma)\mathbb{E}_{q(x_1|x_0, z)}[\log p_{\theta}(x_0|x_1, z)]].\\   
\end{aligned}
\end{equation}

Further more, from triangle inequality we have 

\begin{equation}
\begin{aligned}
&\sum_{t>1} \mathbb{E}_{q(x_t|x_0, z)}[\gamma\frac{||x_0 - f_{\theta}(x_t, t, z)||^2}{2\sigma_t^2}]\\ &\leq\sum_{t>1} \mathbb{E}_{q(x_t|x_0, z)}[\gamma\frac{||x_0 - f_{\text{pre}}(x_t, t, z)||^2+||f_{\text{pre}}(x_t, t, z) - f_{\theta}(x_t, t, z)||^2}{2\sigma_t^2}]    
\end{aligned}
\end{equation}

So another weaker upper bound is given by 
\begin{equation}
\begin{aligned}
\label{weaker_bound}
&\mathrel{\phantom{=}}\mathbb{E}_{p(z)}\mathbb{E}_{p_{\text{pre}}(x_0|z)}[-(r(x_0,z)+\gamma)\log{p_\theta(x_0|z)}]\\
&\leq \mathbb{E}_{p(z)}\mathbb{E}_{p_{\text{pre}}(x_0|z)}[\mathbb{E}_{q(x_T|x_0, z)}[(r(x_0,z)+\gamma)\text{KL}(q(x_T|x_0)\|p(x_T))]\\
&\mathrel{\phantom{=}}+\sum_{t>1} \mathbb{E}_{q(x_t|x_0, z)}[\frac{r(x_0,z)||x_0 - f_{\theta}(x_t, t,z)||^2+\gamma(||x_0-f_{\text{pre}}(x_t, t,z)||^2+||f_{\text{pre}}(x_t, t,z)-f_{\theta}(x_t, t, z)||^2)}{2\sigma_t^2}]\\
&\mathrel{\phantom{=}}-\mathbb{E}_{q(x_1|x_0,z)}[(r(x_0,z)+\gamma)\log p_{\theta}(x_0|z,x_1)]].\\
\end{aligned}   
\end{equation}

To minimize the weighted bound, besides training the diffusion model using the reweighted KL loss, we can meanwhile punish the $L_2$ distance between the direction from pre-trained model and the current model.
% We also try out this weaker bound in experiments and find that it still struggles to achieve both high reward and high fidelity with different choices of the regularization weight, so we only include the tighter bound in both Lemma~\ref{lemma_sup_kl} and our experimental results.

\section{Experimental Details} \label{app:exp}

\paragraph{Online RL training.}For hyper-parameters of online RL training used in Section~\ref{sec:main_exp}., we use $\alpha=10, \beta = 0.01$, learning rate = $10^{-5}$ with other default hyper-parameters in AdamW, sampling batch size $m=10$. For policy gradient training, to perform more gradient steps without the need of re-sampling, we perform $5$ gradient steps per sampling step, with gradient norm clipped to be smaller than $0.1$, and use importance sampling to handle off-policy samples, and use batch size $n = 32$ in each gradient step. We train the models till it generates $20000$ online samples, which matches the number of samples in supervised fine-tuning.
For stable training, we freeze the weights in batch norm to be exactly the same as the pretrained diffusion model. We also explore the use of the ``baseline function'' to reduce the variance during gradient estimation: we fit a value function $V(x_t, t, z)$ to estimate the expected reward of $x_0$ using the current policy. In practice, we find that such value function helps to achieve faster training under the single-prompt setting, but would cause instability in training under the multi-prompt setting. We expect the instability comes from not having enough samples to fit the value function, making the gradient estimation biased and thus causing failure in training. We plan to explore the use of a value function under the multi-prompt setting as future work.
% \ow{Do any of the experiments shown include the value function? If so, we should mention it in the main paper.}-> no they don't appear in the main paper

\paragraph{Supervised training.}

For hyper-parameters of supervised training, we use $\gamma = 1.0$ as the default option in Section~\ref{sec:main_exp},  which is chosen from $\gamma \in \{0.1,1.0,2.0,5.0\}$.
We use learning rate $=2\times 10^{-5}$ with other default hyper-parameters in AdamW, which was chosen from $\{5\times 10^{-6}, 1\times 10^{-5}, 2\times 10^{-5}, 5\times10^{-5}\}.$ 
We use batch size $n=128$ and $M = 20000$ such that both algorithms use the same number of samples.
% For hyper-parameters of supervised training, we use $\gamma = 0.1$ as the default option in Section~\ref{sec:main_exp}\footnote{\textcolor{black}{Ablation study on the choice of $\gamma$ can be found in Appendix~\ref{app: sup_kl}}.},  
% % which is the \textcolor{black}{best configuration? how to define? or omit that?} we found in $\gamma \in \{0.0,0.1,1.0,2.0,5.0\}$, 
% with learning rate $=2\times 10^{-5}$ with other default hyper-parameters in AdamW, which was chosen from $\{5\times 10^{-6}, 1\times 10^{-5}, 2\times 10^{-5}, 5\times10^{-5}\}.$ We use batch size \textcolor{black}{$n=128$} and $M = 20000$ such that both algorithms use the same number of samples.
Notice that Lemma~\ref{lemma_sup_kl} requires $r+\gamma$ to be non-negative, we apply a filter of reward such that if $r+\gamma <0$, we just set it to 0. In practice, we also observe that without this filtering, supervised fine-tuning could fail during training, which shows that our assumption is indeed necessary.

\section{Investigation on ImageReward} \label{app:imagereward}

\textcolor{black}{We investigate the quality of ImageReward~\cite{imagereward} by evaluating its prediction of the assessments of human labelers. Similar to \citet{lee2023aligning}, we check whether ImageReward generates a higher score for images preferred by humans. Our evaluation encompasses four text prompt categories: color, count, location, and composition. To generate prompts, we combine words or phrases from each category with various objects. These prompts are then used to generate corresponding images using a pre-trained text-to-image model. We collect binary feedback from human labelers on the image-text dataset and construct comparison pairs based on this feedback. Specifically, we utilize 804, 691, 1154, and 13228 comparison pairs obtained from 38, 29, 41, and 295 prompts for color, location, count, and composition, respectively.\footnote{We attached the full list of text prompts in Supplementary Material ({\tt prompts.csv}).} Additionally, for evaluation of complex text prompts from human users, we also utilize the test set from ImageReward, which consists of 6399 comparison pairs from 466 prompts.\footnote{\href{https://github.com/THUDM/ImageReward/blob/main/data/test.json}{https://github.com/THUDM/ImageReward/blob/main/data/test.json}} Table~\ref{table:tfa} compares the accuracy of ImageReward and baselines like CLIP~\cite{clip} and BLIP~\cite{blip} scores, which justifies the choice of using ImageReward for fine-tuning text-to-image models.}

\begin{table}[h]
\begin{center}
\small
\begin{tabular}{l|ccccc}
\toprule
& Color & Count & Location & Composition & Complex\\
\midrule
CLIP & 82.46 & 66.11 & $\mathbf{80.60}$ & 70.98 & 54.83 \\
BLIP & 77.36 & 61.61 & 78.14 & 70.98 & 57.79 \\
ImageReward & $\mathbf{86.06}$ & $\mathbf{73.65}$ & $79.73$ & $\mathbf{79.65}$ & $\mathbf{65.13}$ \\
\bottomrule
\end{tabular}
\end{center}
\caption{\textcolor{black}{Accuracy (\%) of CLIP score, BLIP score and ImageReward when predicting the assessments of human labelers.}}
\label{table:tfa}
\end{table}

\section{More Results from RL Training}
\label{app:multiprompt}
\subsection{Multi-prompt training}

\textcolor{black}{We verify the effectiveness of the proposed techniques in enhancing the performance of the text-to-image model fined-tuned on multiple prompts simultaneously. For fine-tuning, we use four text prompts (i.e., ``A green colored rabbit'', ``A cat and a dog'', ``Four wolves in the park'', and ``A dog on the moon''), which are used in Section~\ref{sec:main_exp}. For evaluation, we report the average ImageReward and Aesthetic scores across 200 images (50 images per each prompt).
Table~\ref{table:multiple} shows that RL fine-tuning is more effective than supervised fine-tuning in improving both ImageReward and aesthetic scores across multiple prompts. However, we find that the ImageReward score of the fine-tuned model on multiple prompts (Multi) is a bit lower than the average score of fine-tuned models on a single prompt (Single). We expect that this is due to the varying difficulty of each text prompt, which can pose additional challenges such as gradient conflict as observed in multi-task RL. We defer further investigation of fine-tuning on multiple prompts to future work.}

\begin{table}[t!]
\begin{center}
\small
\begin{tabular}{l|c|cc|cc}
\toprule
& \multirow{2}{*}{\begin{tabular}[c]{@{}c@{}} {Original model}  \end{tabular}} 
& \multicolumn{2}{c|}{SFT model} 
& \multicolumn{2}{c}{RL model}  \\ 
& &  {Single} & {Multi} &  {Single} & {Multi}  \\
\midrule
ImageReward score & 0.23 & 0.94 & 0.88 & 1.25 & 1.10 \\
Aesthetic score & 5.61 & 5.27 & 5.30 & 5.68 & 5.70 \\
\bottomrule
\end{tabular}
\end{center}
\caption{\textcolor{black}{ImageReward scores and Aesthetic scores from the original model, supervised fine-tuned (SFT) model, and RL fine-tuned model, all are trained on four text prompts simultaneously. We report the average ImageReward and Aesthetic scores across 200 images (50 images per each prompt). For SFT and RL models, we also provide the average performance of fine-tuned models trained on single prompts (Single) for comparison.}}
\label{table:multiple}
\end{table}

We also report details for multi-prompt training. We still use the learning rate $10^{-5}$ as the single prompt setting, but increase the batch size per sampling step to $n=128$ for stable training. Also, we train for a longer time for multi-prompt such that it utilizes $50000$ online samples.

\subsection{Long and complex prompts}
We show that our method not only works for short and simple prompts like "A green colored rabbit", but can also work with long and complex prompts. For example, in Fig.~\ref{fig:six} we adopt a complex prompt and compare the images generated by the original model and the supervised fine-tuned model. We can observe that online training encourages the models to have a different style of painting with more fine-grained details, which is generally hard to achieve by supervised fine-tuning only.
\begin{figure} [h] \centering
\includegraphics[width=.99\textwidth]{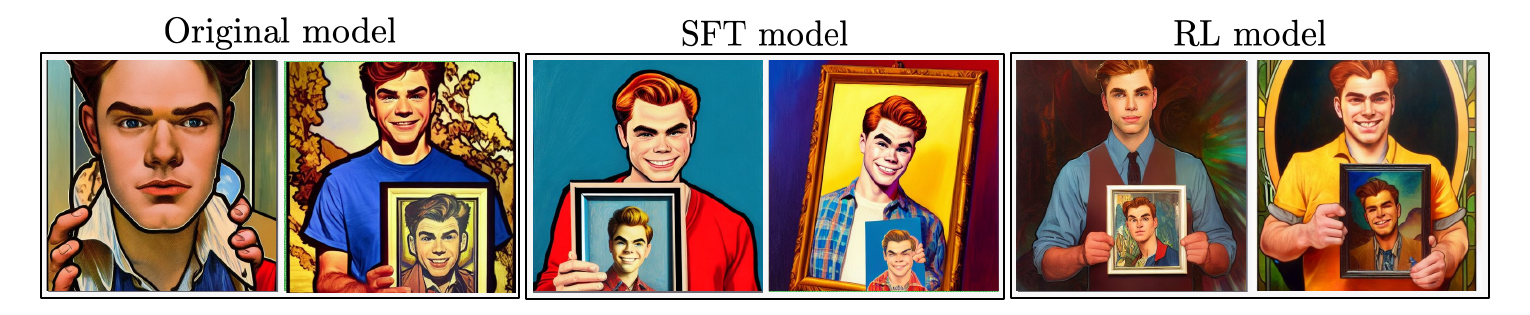}
\caption{Text prompt: "oil portrait of archie andrews holding a picture of among us, intricate, elegant, highly detailed, lighting, painting, artstation, smooth, illustration, art by greg rutowski and alphonse mucha".}
\label{fig:six}
\end{figure}

\section{Ablation Study on KL Regularization in Supervised Fine-Tuning}
\label{app: sup_kl}

% \paragraph{KL regularization with a tighter bound}

% In Lemma~\ref{lemma_sup_kl}, we introduce KL regularization (eq.~(\ref{tighter_bound})) for supervised fine-tuning, which can be implemented by shifting the original reward by $\gamma$ during training with the reward weighted loss. In this section, we also consider another stronger KL regularization presented in Appendix~\ref{app: sup_kl} as eq.~(\ref{weaker_bound}). (we denote it as a stronger regularization in the sense that it is an upper bound of the regularization term we consider in eq.~\ref{tighter_bound}). \textcolor{black}{This strong KL regularization can be implemented by adding an extra term during normal training reward-weighted loss: add an extra punishment of the $L_2$ distance between the denoising directions from the pre-trained model and the current model. }

In Lemma~\ref{lemma_sup_kl}, we introduce KL regularization (eq.~(\ref{tighter_bound})) for supervised fine-tuning, which can be incorporated by adjusting the original reward with a shift factor $\gamma$ in the reward-weighted loss. 
We refer to this regularization as KL-D since it is based only on data from the pre-trained model.

In this section, we also consider another KL regularization presented in Appendix~\ref{app: sup_kl} as eq.~(\ref{weaker_bound}). This KL regularization can be implemented by introducing an additional term in the reward-weighted loss. This extra term penalizes the $L_2$ distance between the denoising directions derived from the pre-trained model and the current model. We refer to it as KL-O because it also regularizes the output from the current model to be close to that from the pre-trained model.

% In this section, besides the KL regularization in eq.~(\ref{tighter_bound}) which is presented in Lemma~\ref{lemma_sup_kl} (can be implemented by shifting the original reward by $\gamma$ during training with the reward reweighted loss), we also consider another stronger KL regularization presented in Appendix~\ref{app: sup_kl} as eq.~(\ref{weaker_bound}) (can be implemented by adding an extra term to punish the $L_2$ distance between the direction from pre-trained model and the current model during normal training with the reweighted loss). 

We present the effects of both KL-D and KL-O with different KL coefficients $\gamma \in \{0.1,1.0,2.0,5.0\}$ in Figure~\ref{fig: im_as_sup_ablation_rabbit} and Figure~\ref{fig: sup_kl_ablation}.
We observe the followings:
% We sweep $\gamma \in \{0.1,1.0,2.0,5.0\}$ for both options,
% and present ImageReward vs Aesthetic score trade-off in Figure~\ref{fig: im_as_sup_ablation_rabbit} and visualization of the generated samples in Figure~\ref{fig: sup_kl_ablation}.
% From both Figure~\ref{fig: im_as_sup_ablation_rabbit} and Figure~\ref{fig: sup_kl_ablation}, we can observe that
\begin{itemize} [leftmargin=7mm]
    \item \textcolor{black}{KL-D (eq.~(\ref{tighter_bound})) can increase the aesthetic score. However, even with a large value of $\gamma$, it does not yield a significant improvement in visual quality. Moreover, it tends to result in lower ImageReward scores overall.}
    % The weak KL regularization (eq.~(\ref{tighter_bound})), employed in the main paper, can increase the aesthetic score but there is no significant improvement in visual quality even if $\gamma$ is large, while it would also generally suffer from lower ImageReward scores.

    \item \textcolor{black}{In Figure~\ref{fig: sup_kl_ablation}, it is evident that KL-O is more noticeably effective in addressing the failure modes in supervised fine-tuning (SFT) compared to KL-D, especially when $\gamma$ is relatively large. However, as a tradeoff, KL-O significantly reduces the ImageReward scores.}
    %From Figure~\ref{fig: sup_kl_ablation}, the strong KL regularization is more visibly effective to solve the failure modes in SFT than weak KL regularization when $\gamma$ is relatively large. However, it sacrifices the ImageReward scores similar to weak KL regularization.

    \item \textcolor{black}{In general, achieving both high ImageReward and aesthetic scores simultaneously is challenging for supervised fine-tuning (SFT), unlike RL fine-tuning (blue bar in Figure~\ref{fig: im_as_sup_ablation_rabbit}).} 
    % In general, it is hard for SFT to attain ImageReward and aesthetic scores both as high unlike RL fine-tuning (one might refer to ImageReward and aesthetic scores we present in Section~\ref{sec:main_exp}).
\end{itemize}

\begin{figure*} [h!] \centering
\subfigure[ImageReward score]
{\includegraphics[width=0.435\textwidth]{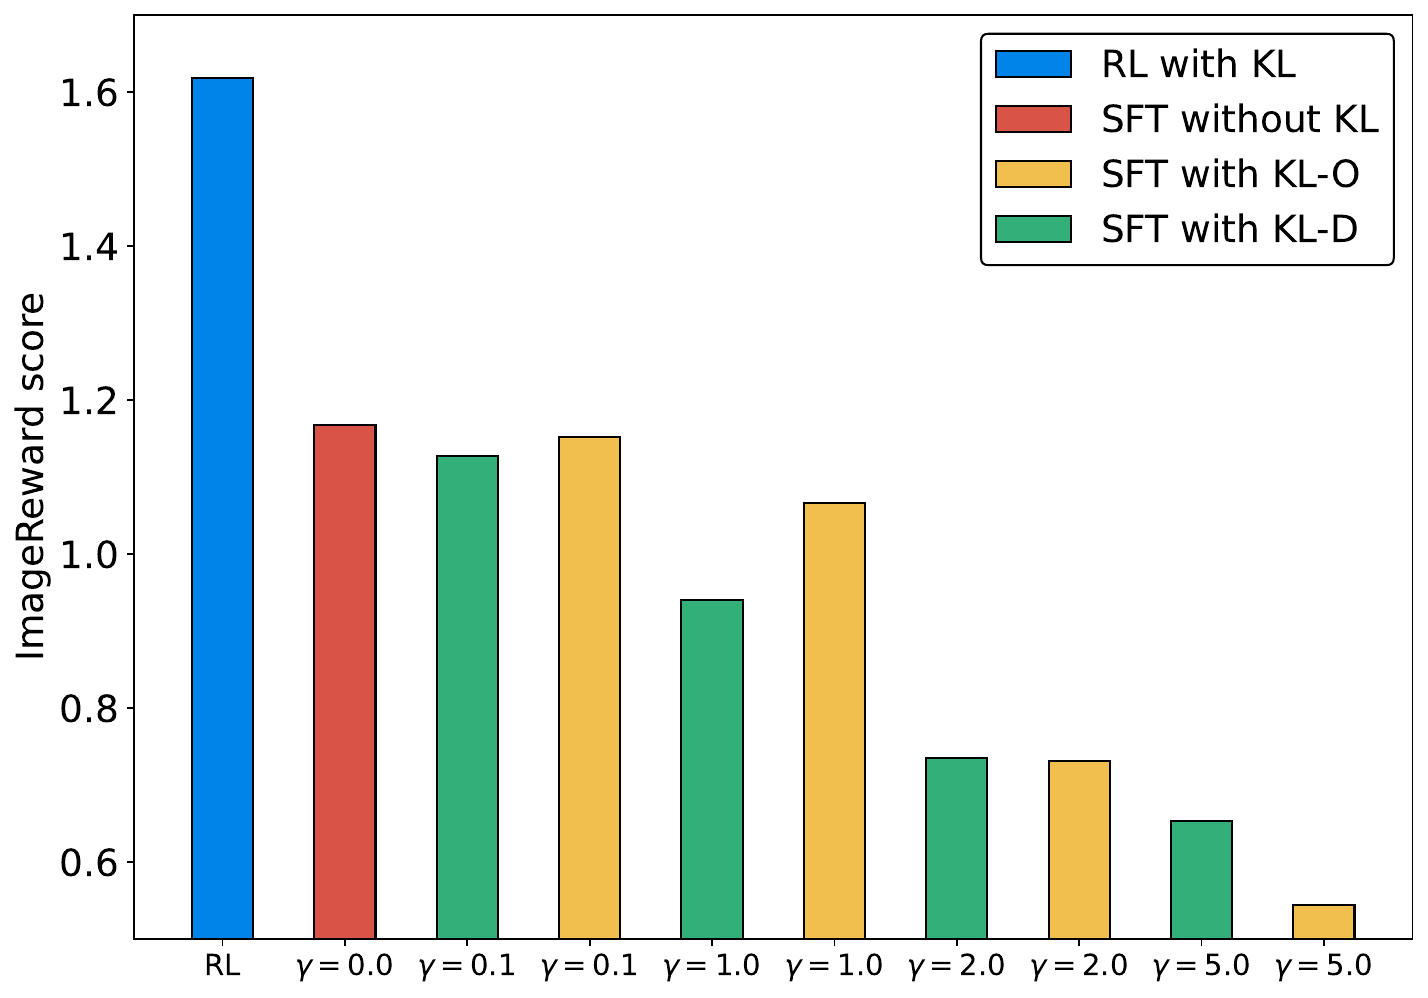}} 
\subfigure[Aesthetic score]
{\includegraphics[width=0.45\textwidth]{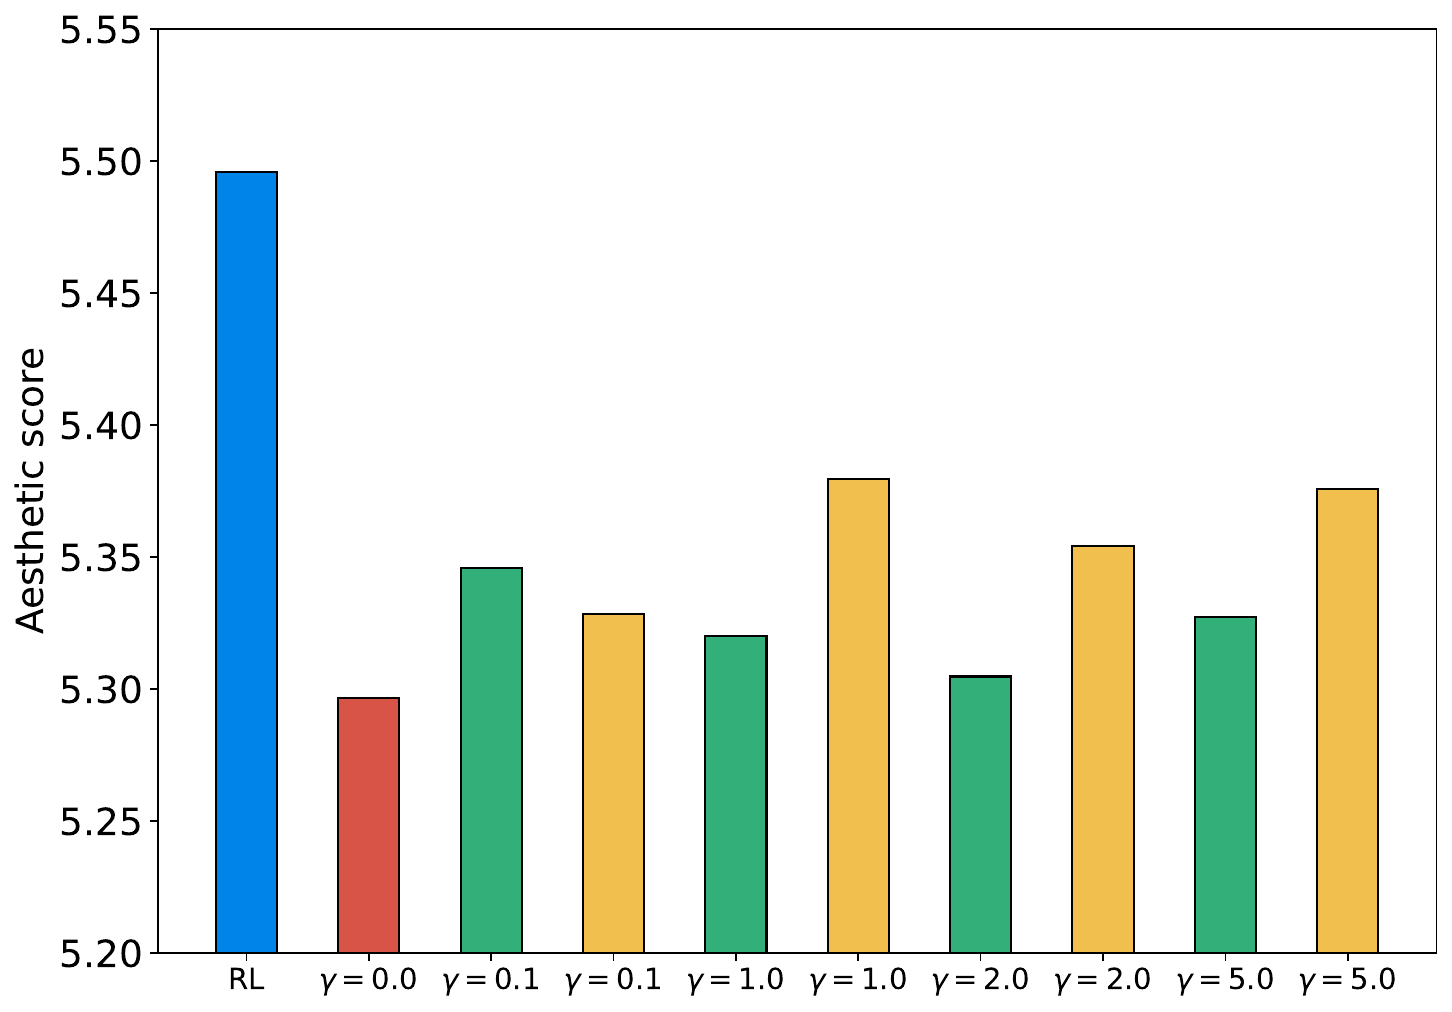}}
% \label{fig}
\caption{(a) ImageReward scores and (b) Aesthetic scores of supervised fine-tuned (SFT) models with different choices of regularization term and coefficient ($\gamma$) on text prompt "A green colored rabbit". Each score is averaged over 50 samples from each model. KL-O and KL-D refer to eq.~(\ref{weaker_bound}) and eq.~(\ref{tighter_bound}), respectively.}
%KL ablation in supervised fine-tuning using the single prompt "A green colored rabbit", with different choices of regularization term and weight. Each score is averaged over 50 samples from each model.}
\label{fig: im_as_sup_ablation_rabbit}
\end{figure*}

\begin{figure} [h] \centering
\includegraphics[width=.9\textwidth]{figures/sup_kl_rabbit.pdf}
\caption{Samples from supervised fine-tuned models with different choices of regularization term and coefficient ($\gamma$) on ``A green colored rabbit".}
\label{fig: sup_kl_ablation}
\end{figure}

\begin{figure*} [h!] \centering
\subfigure[``A green colored rabbit"]
{\includegraphics[width=0.85\textwidth]{figures/sup_kl_rabbit.pdf}
% \label{fig}
} 
\subfigure[``Four wolves in the park"]
{\includegraphics[width=0.85\textwidth]{figures/sup_kl_wolves.pdf}
% \label{fig}
}
\subfigure[``A cat and a dog"]
{\includegraphics[width=0.85\textwidth]{figures/sup_kl_cat.pdf}
% \label{fig}
}
\subfigure[``A dog on the moon"]
{\includegraphics[width=0.85\textwidth]{figures/sup_kl_dog.pdf}
% \label{fig}
}
\caption{Samples from supervised fine-tuned models with different KL regularization and KL coefficients.}
\label{fig: sup_kl_ablation}
\end{figure*}

\begin{figure*} [h!] \centering
\subfigure[ImageReward for SFT models]
{\includegraphics[width=0.4\textwidth]{figures/reward_kl_sup_four_wolves.pdf}
% \label{fig}
} 
\hfill
\subfigure[Aesthetic score for SFT models]
{\includegraphics[width=0.4\textwidth]{figures/aes_kl_sup_four_wolves.pdf}}
% \label{fig}
\caption{KL ablation in supervised fine-tuning using the single prompt "Four wolves in the park", with different choices of regularization term and weight.}
\label{fig: im_as_sup_ablation_wolves}
\end{figure*}

\begin{figure*} [h!] \centering
\subfigure[ImageReward for SFT models]
{\includegraphics[width=0.4\textwidth]{figures/reward_kl_sup_cat_dog.pdf}
% \label{fig}
} 
\hfill
\subfigure[Aesthetic score for SFT models]
{\includegraphics[width=0.4\textwidth]{figures/aes_kl_sup_cat_dog.pdf}}
% \label{fig}
\caption{KL ablation in supervised fine-tuning using the single prompt "A cat and a dog", with different choices of regularization term and weight.}
\label{fig: im_as_sup_ablation_cat_dog}
\end{figure*}

\begin{figure*} [h!] \centering
\subfigure[ImageReward for SFT models]
{\includegraphics[width=0.4\textwidth]{figures/reward_kl_sup_dog_moon.pdf}
% \label{fig}
} 
\hfill
\subfigure[Aesthetic score for SFT models]
{\includegraphics[width=0.4\textwidth]{figures/aes_kl_sup_dog_moon.pdf}}
% \label{fig}
\caption{KL ablation in supervised fine-tuning using the single prompt "A dog on the moon", with different choices of regularization term and weight.}
\label{fig: im_as_sup_ablation_dog_moon}
\end{figure*}

\begin{figure*} [h!] \centering
\subfigure[``A green colored rabbit"]
{\includegraphics[width=0.85\textwidth]{figures/sup_kl_rabbit.pdf}
% \label{fig}
} 
\subfigure[``Four wolves in the park"]
{\includegraphics[width=0.85\textwidth]{figures/sup_kl_wolves.pdf}
% \label{fig}
}
\subfigure[``A cat and a dog"]
{\includegraphics[width=0.85\textwidth]{figures/sup_kl_cat.pdf}
% \label{fig}
}
\subfigure[``A dog on the moon"]
{\includegraphics[width=0.85\textwidth]{figures/sup_kl_dog.pdf}
% \label{fig}
}
\caption{Samples from supervised fine-tuned models with different KL regularization and KL coefficients.}
\label{fig: sup_kl_ablation}
\end{figure*}

\section{More Samples for Qualitative Comparison}
Here we provide more samples from the experiments in Section~\ref{sec:main_exp} and Section~\ref{sec:kl_abl}: see Figure~\ref{fig:app_color}, Figure~\ref{fig:app_comp}, Figure~\ref{fig:app_count}, Figure~\ref{fig:app_loc}, Figure~\ref{fig:app_kl_rl} and Figure~\ref{fig:app_kl_sup}.

\begin{figure*} [h!] \centering
\subfigure[Original model]
{\includegraphics[width=0.99\textwidth]{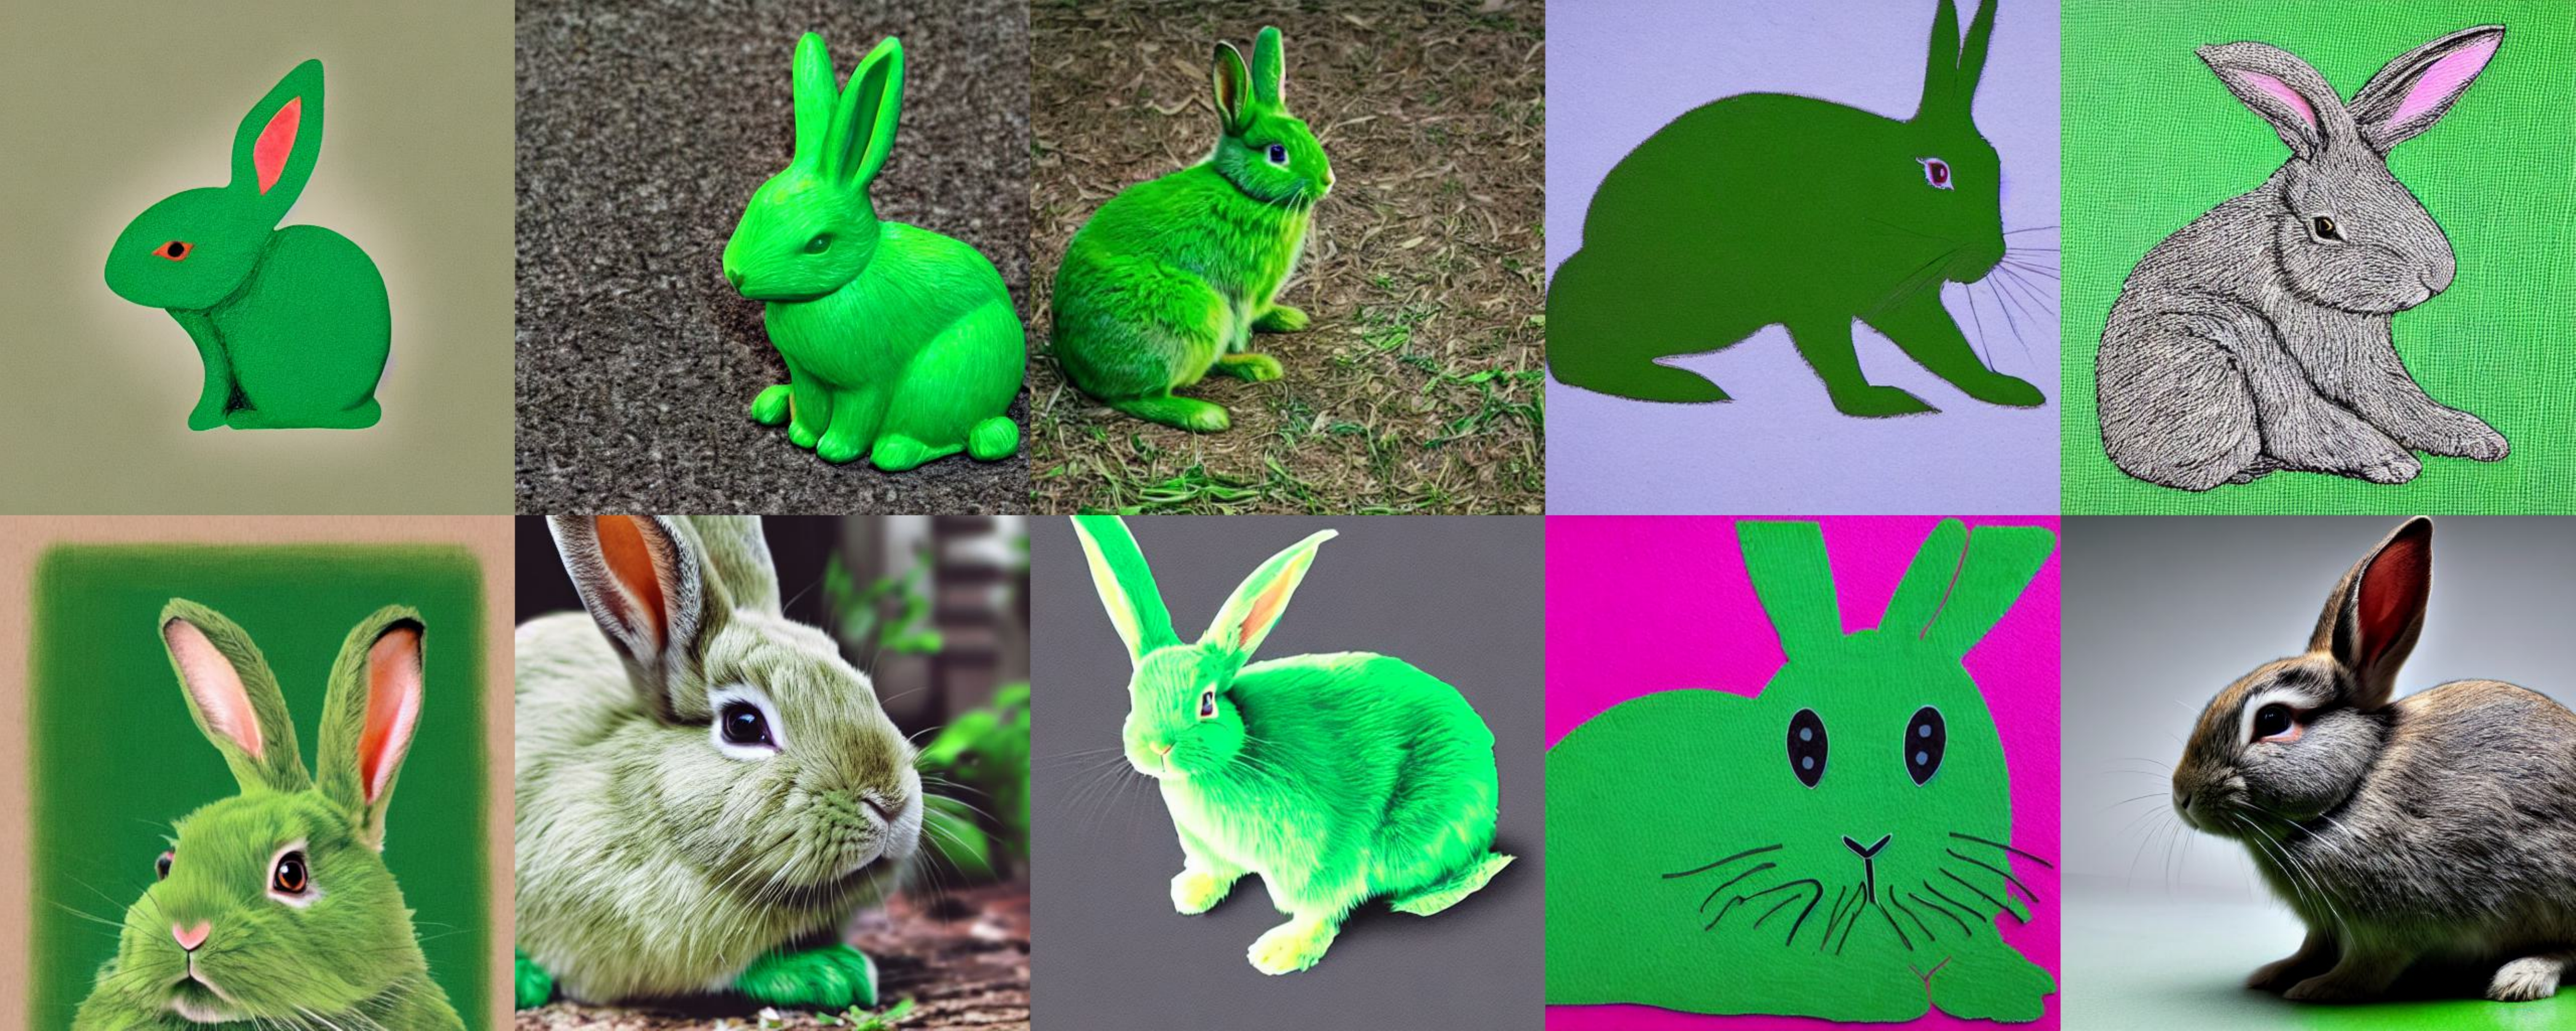}
\label{fig:app_color_0}} 
\subfigure[SFT model]
{\includegraphics[width=0.99\textwidth]{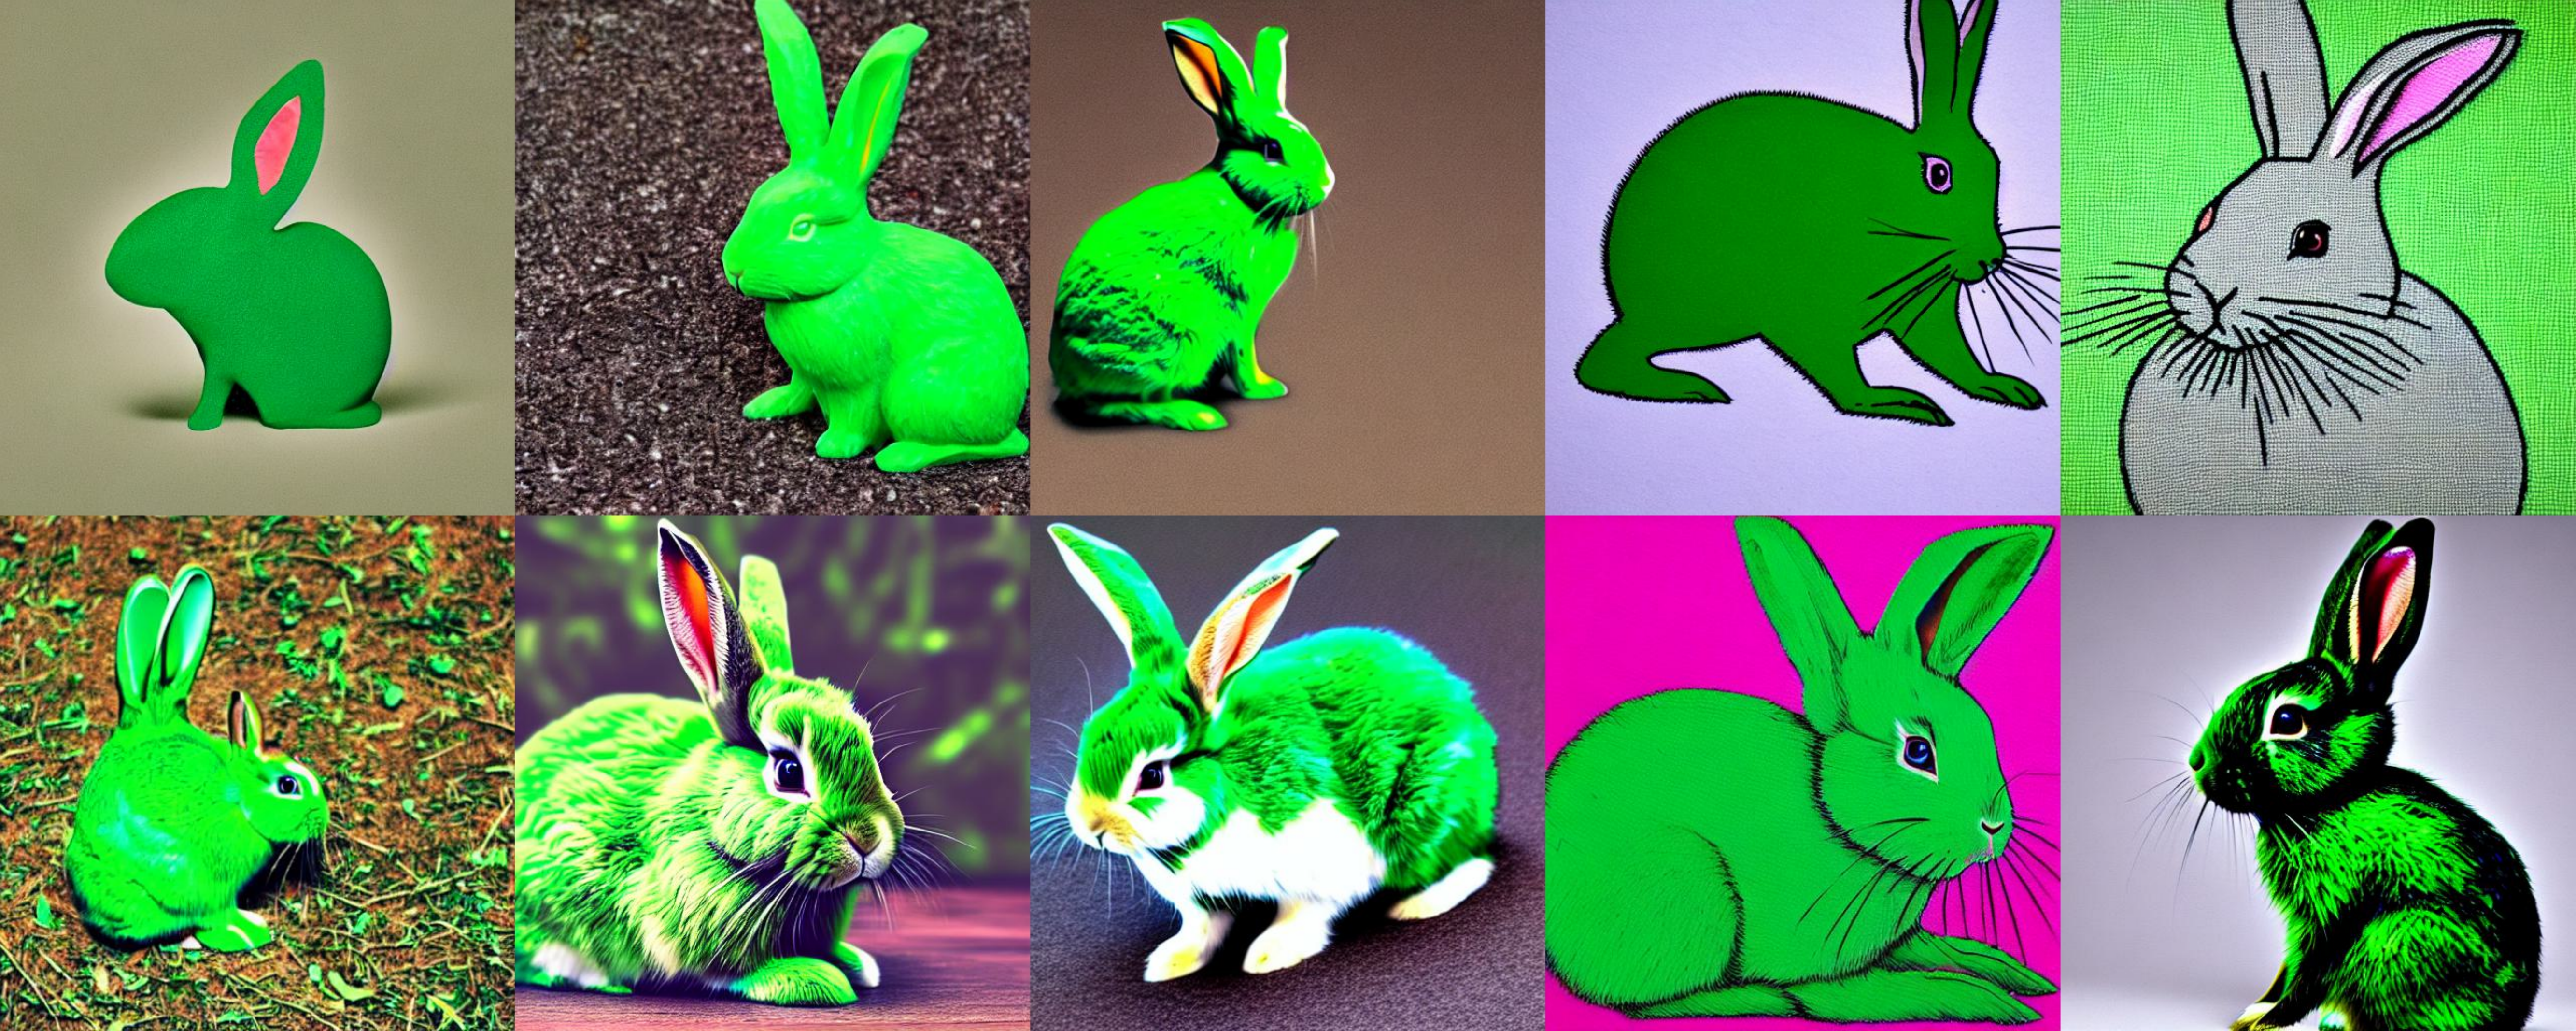}
\label{fig:app_color_1}}
\subfigure[RL model]
{\includegraphics[width=0.99\textwidth]{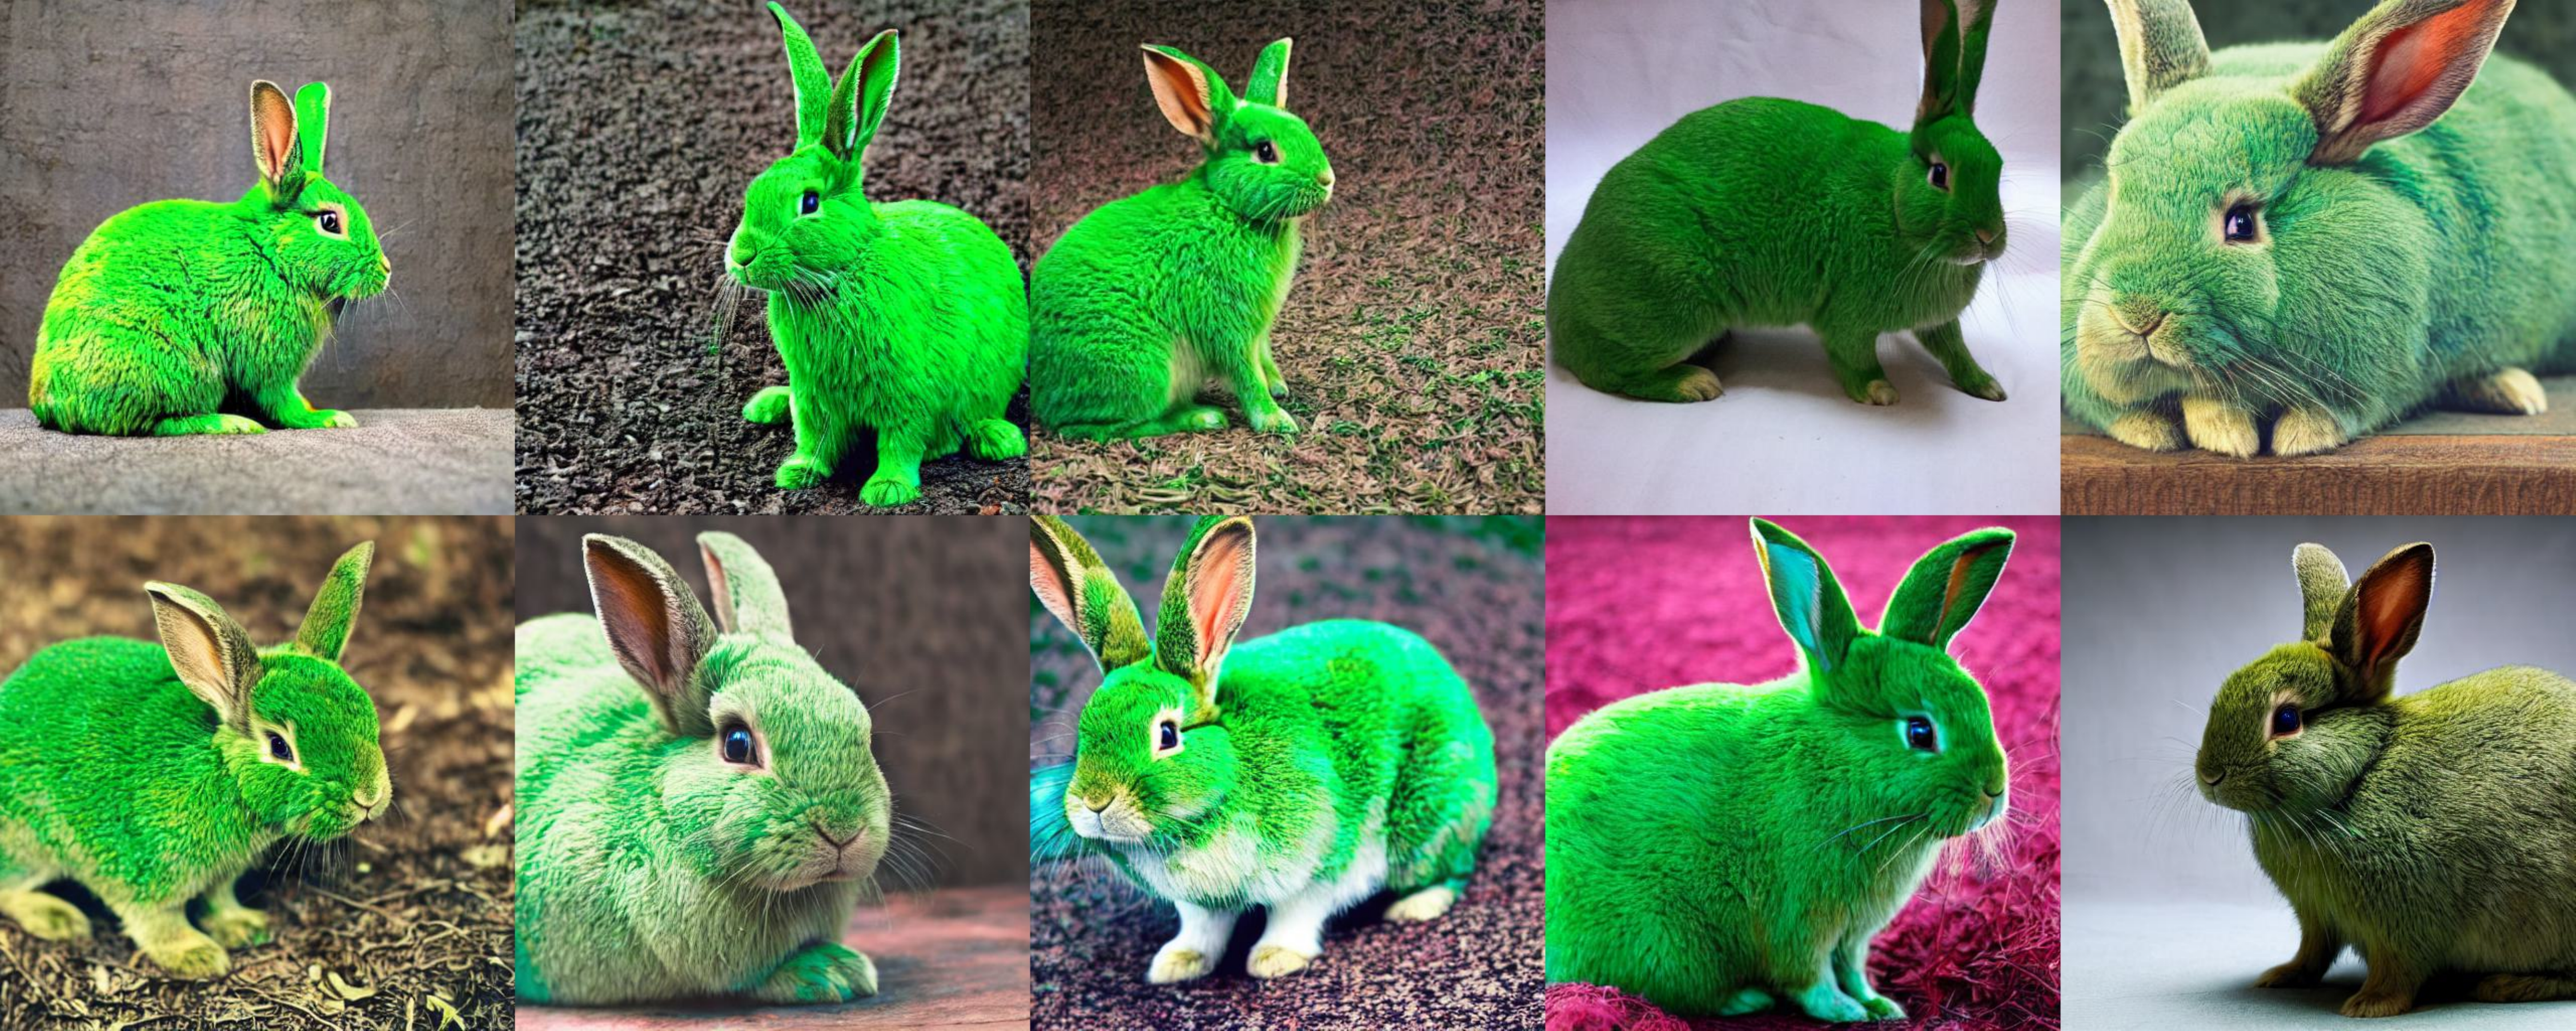}
\label{fig:app_color_2}}
\caption{Non-cherry-picked samples from (a) the original Stable Diffusion model, (b) supervised fine-tuned (SFT) model and (c) RL fine-tuned model.}
\label{fig:app_color}
\end{figure*}

\begin{figure*} [h!] \centering
\subfigure[Original model]
{\includegraphics[width=0.99\textwidth]{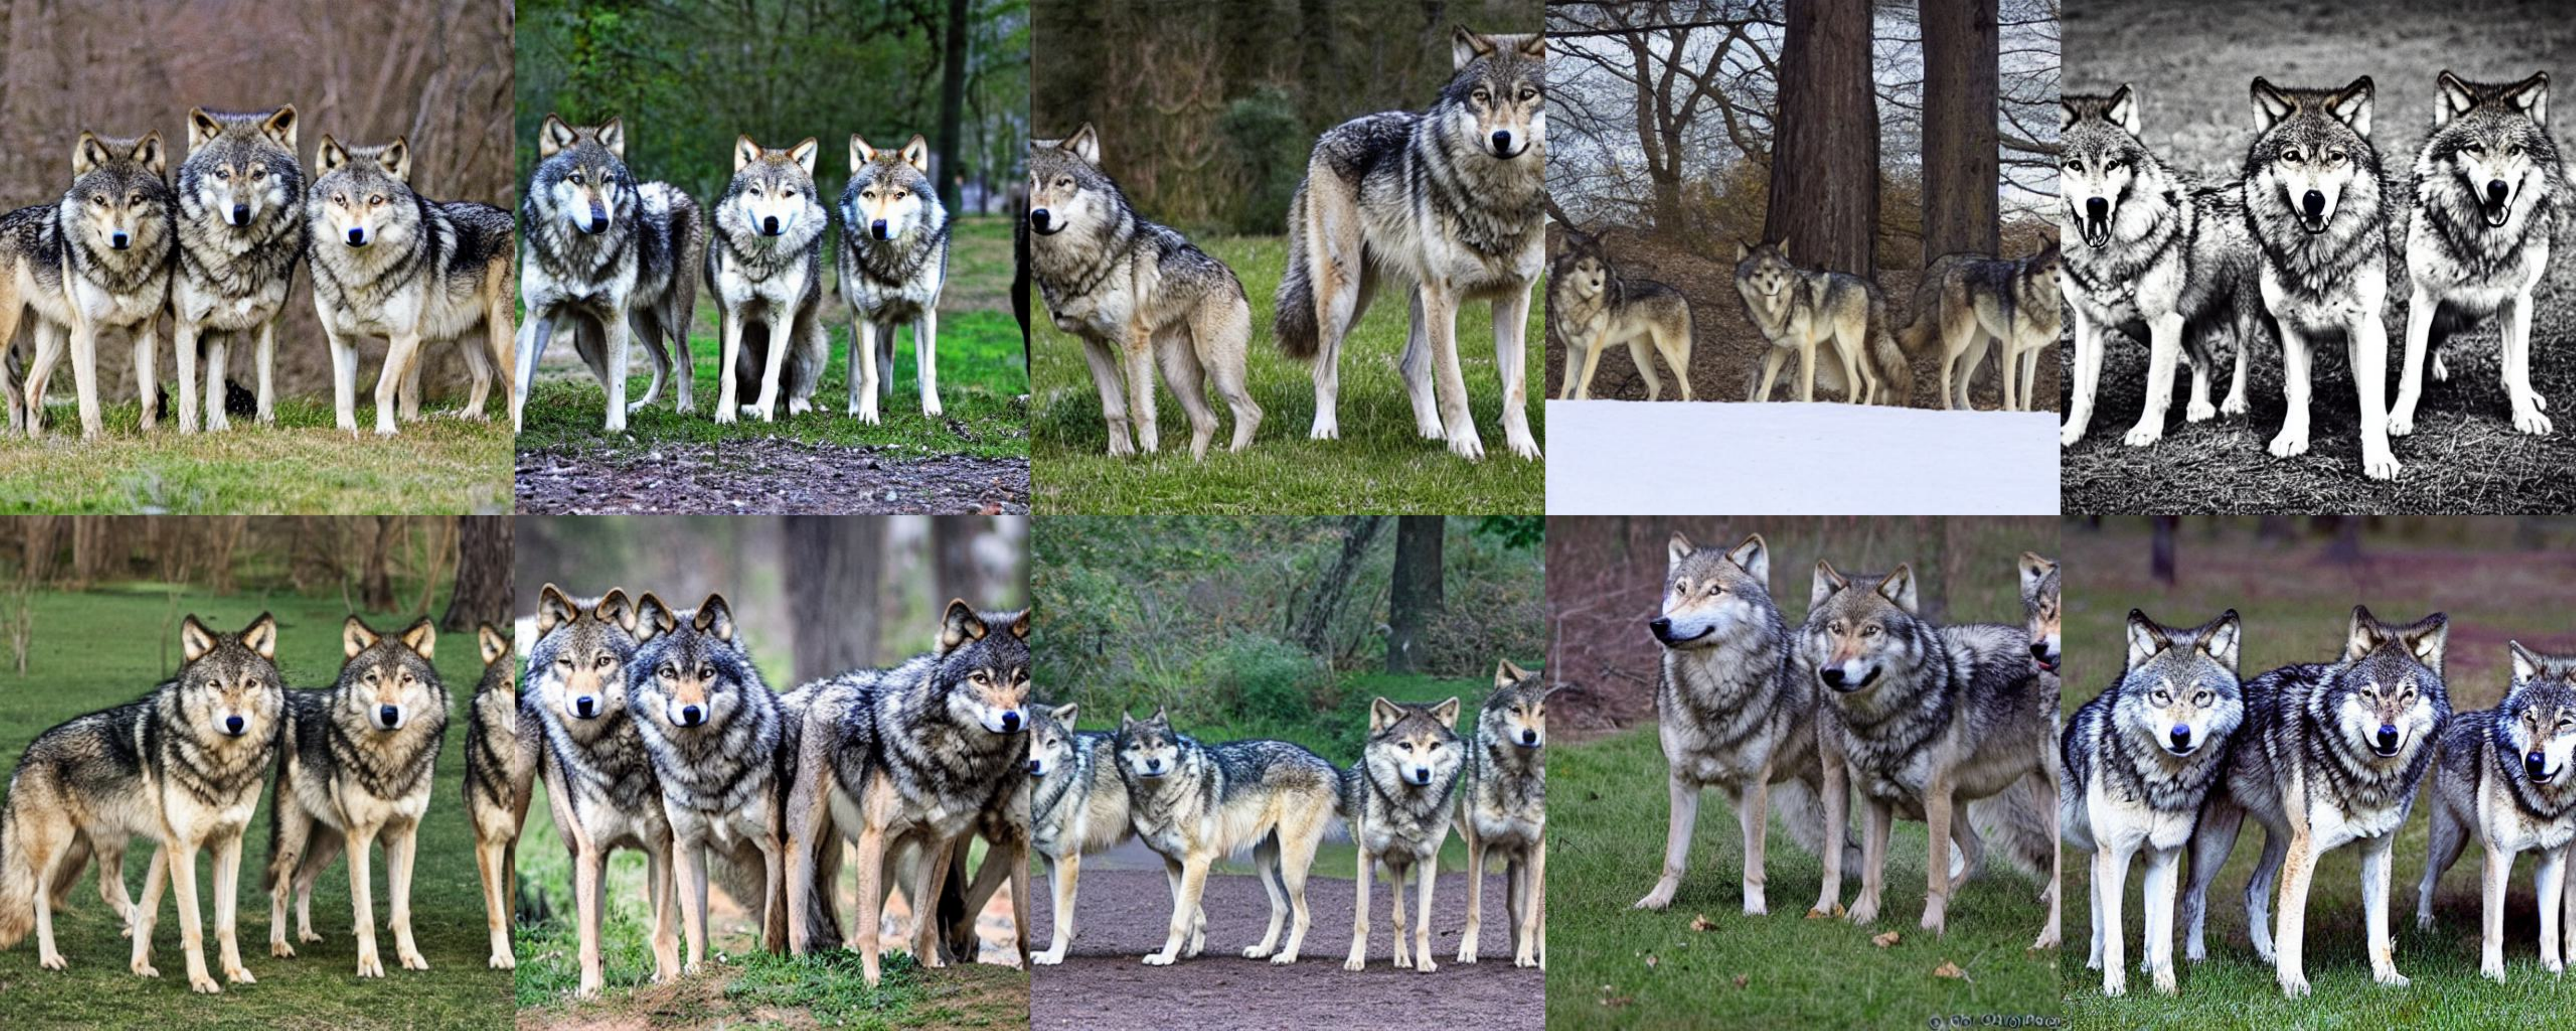}
\label{fig:app_count_0}} 
\subfigure[SFT model]
{\includegraphics[width=0.99\textwidth]{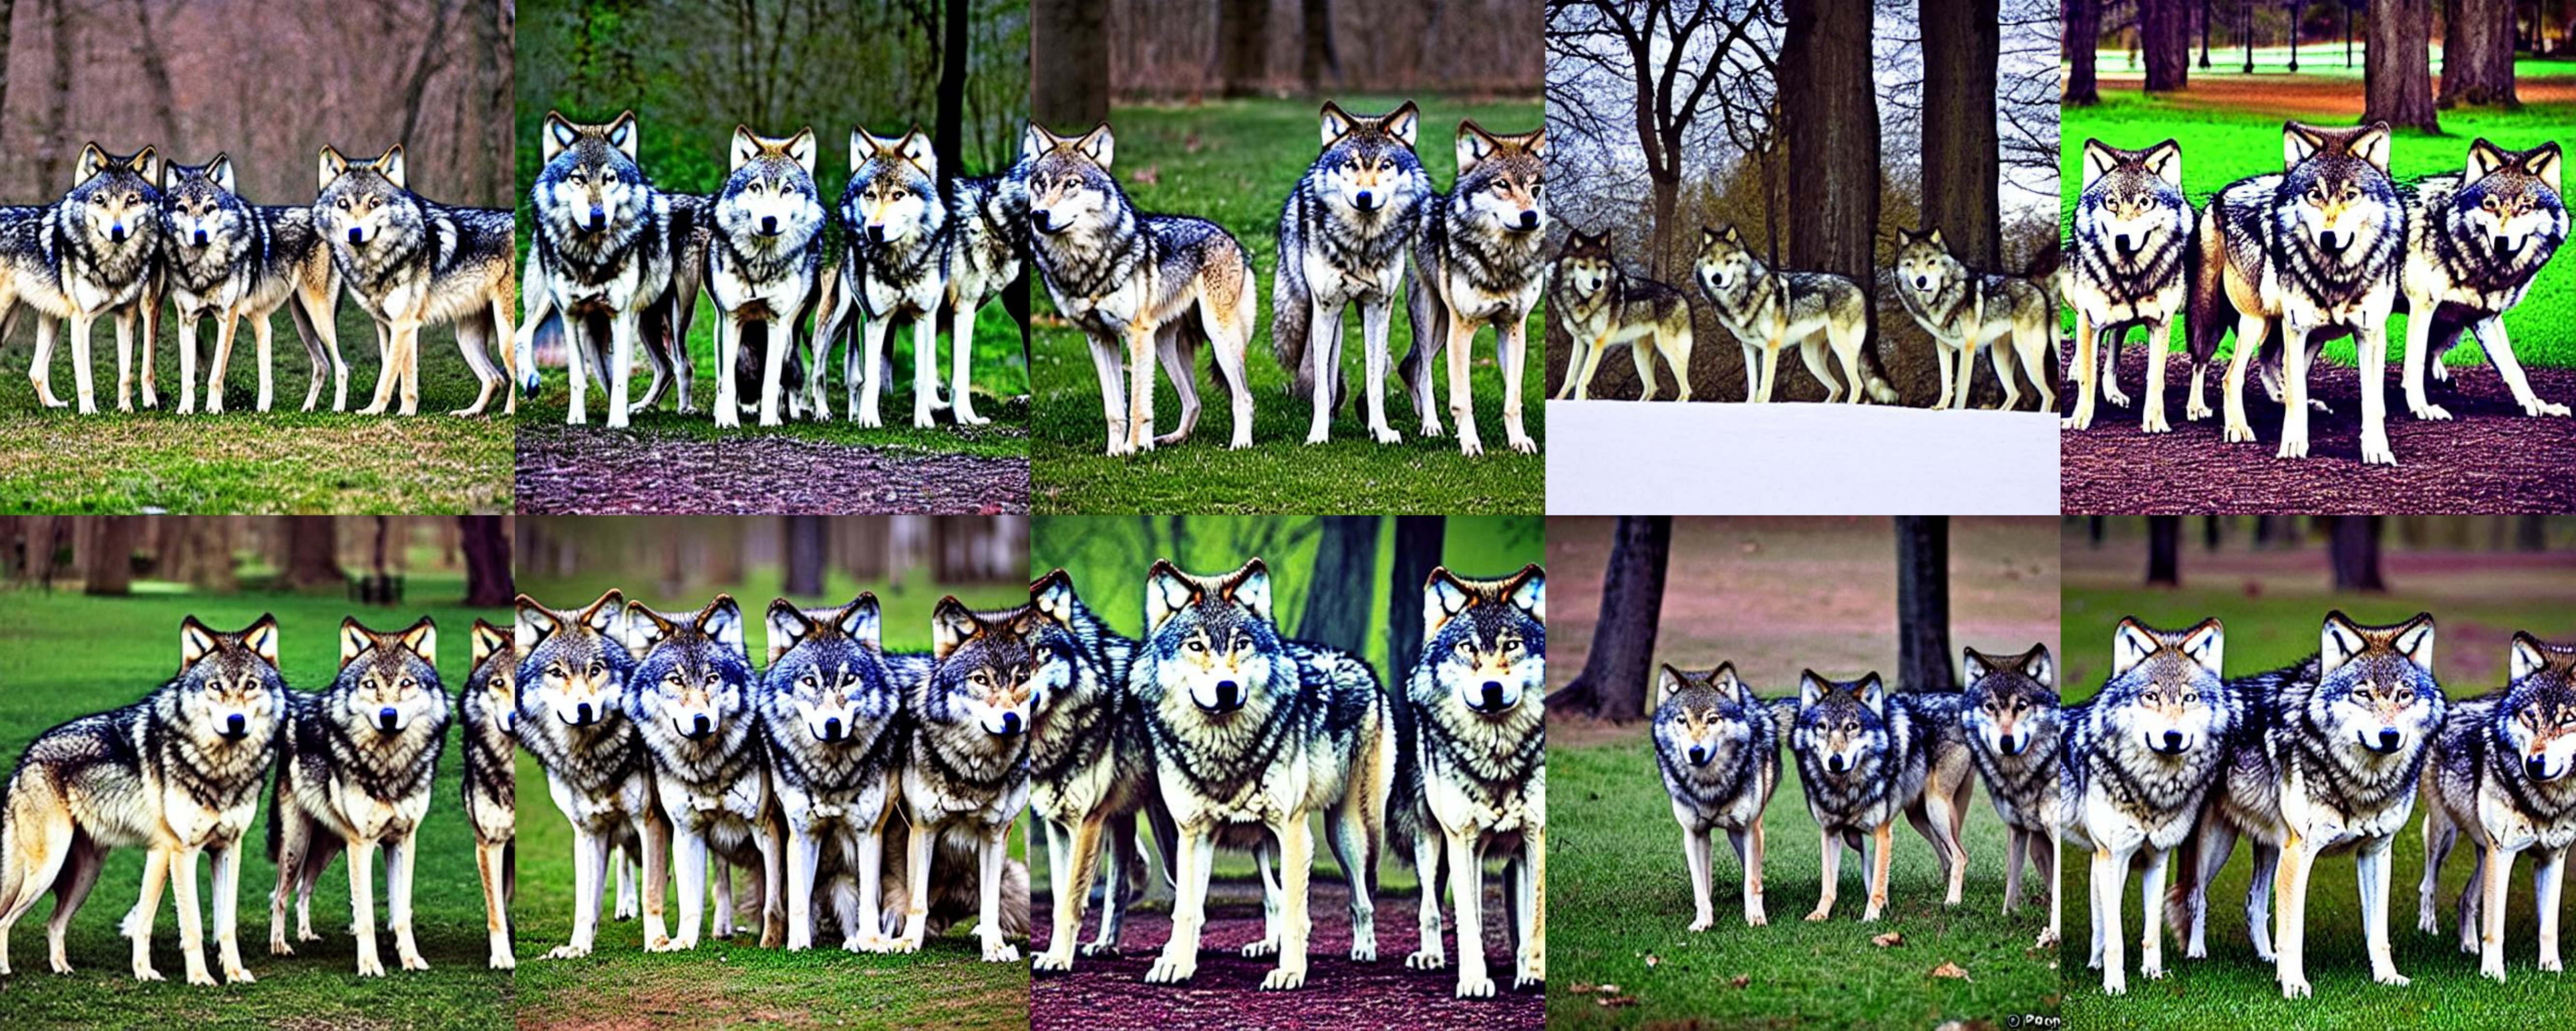}
\label{fig:app_count_1}}
\subfigure[RL model]
{\includegraphics[width=0.99\textwidth]{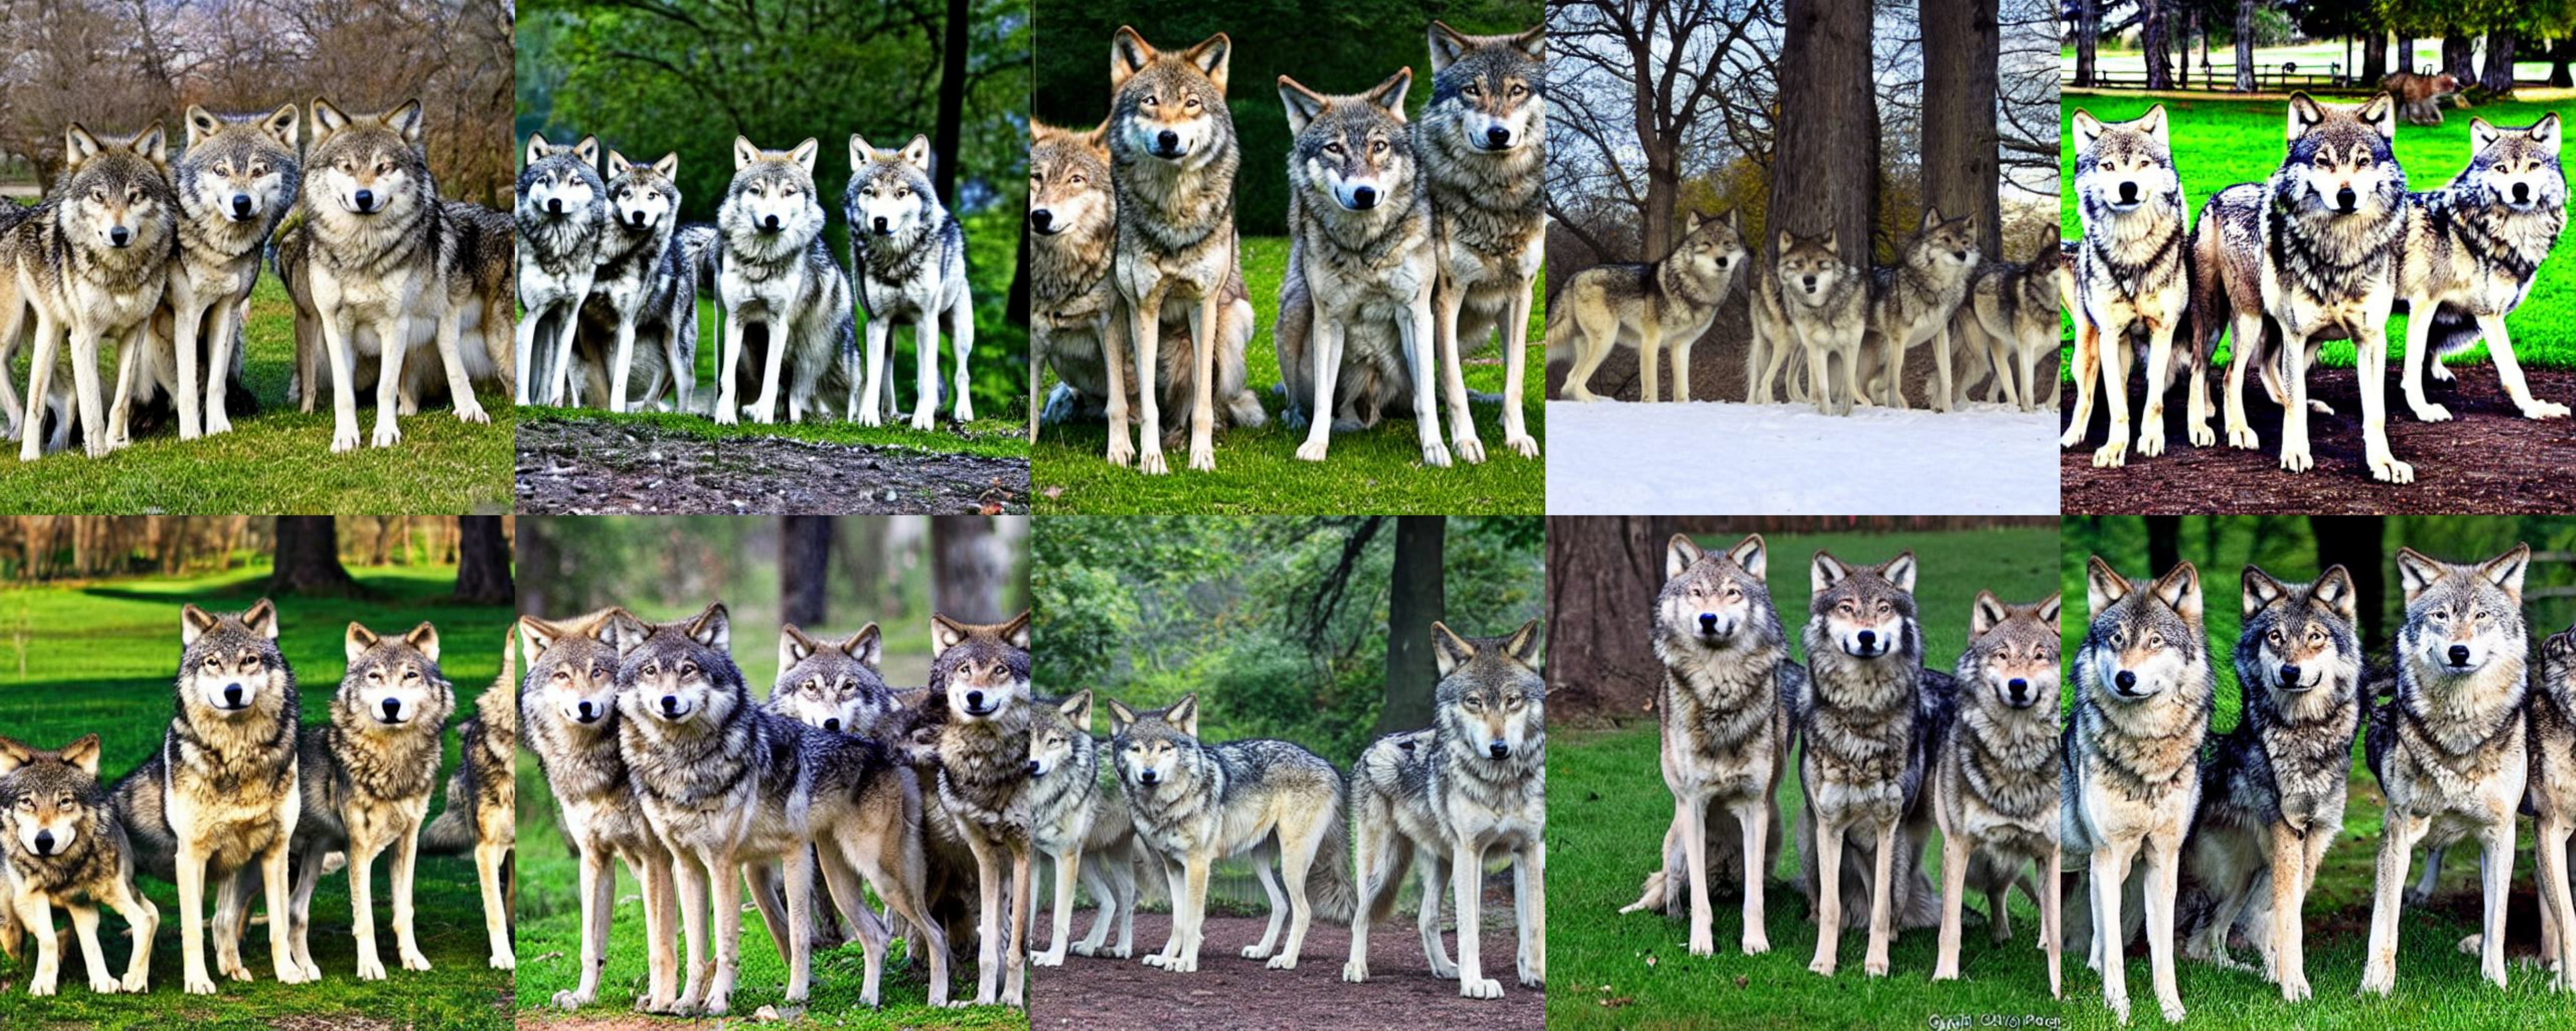}
\label{fig:app_count_2}}
\caption{Non-cherry-picked samples from (a) the original Stable Diffusion model, (b) supervised fine-tuned (SFT) model and (c) RL fine-tuned model.}
\label{fig:app_count}
\end{figure*}

\begin{figure*} [h!] \centering
\subfigure[Original model]
{\includegraphics[width=0.99\textwidth]{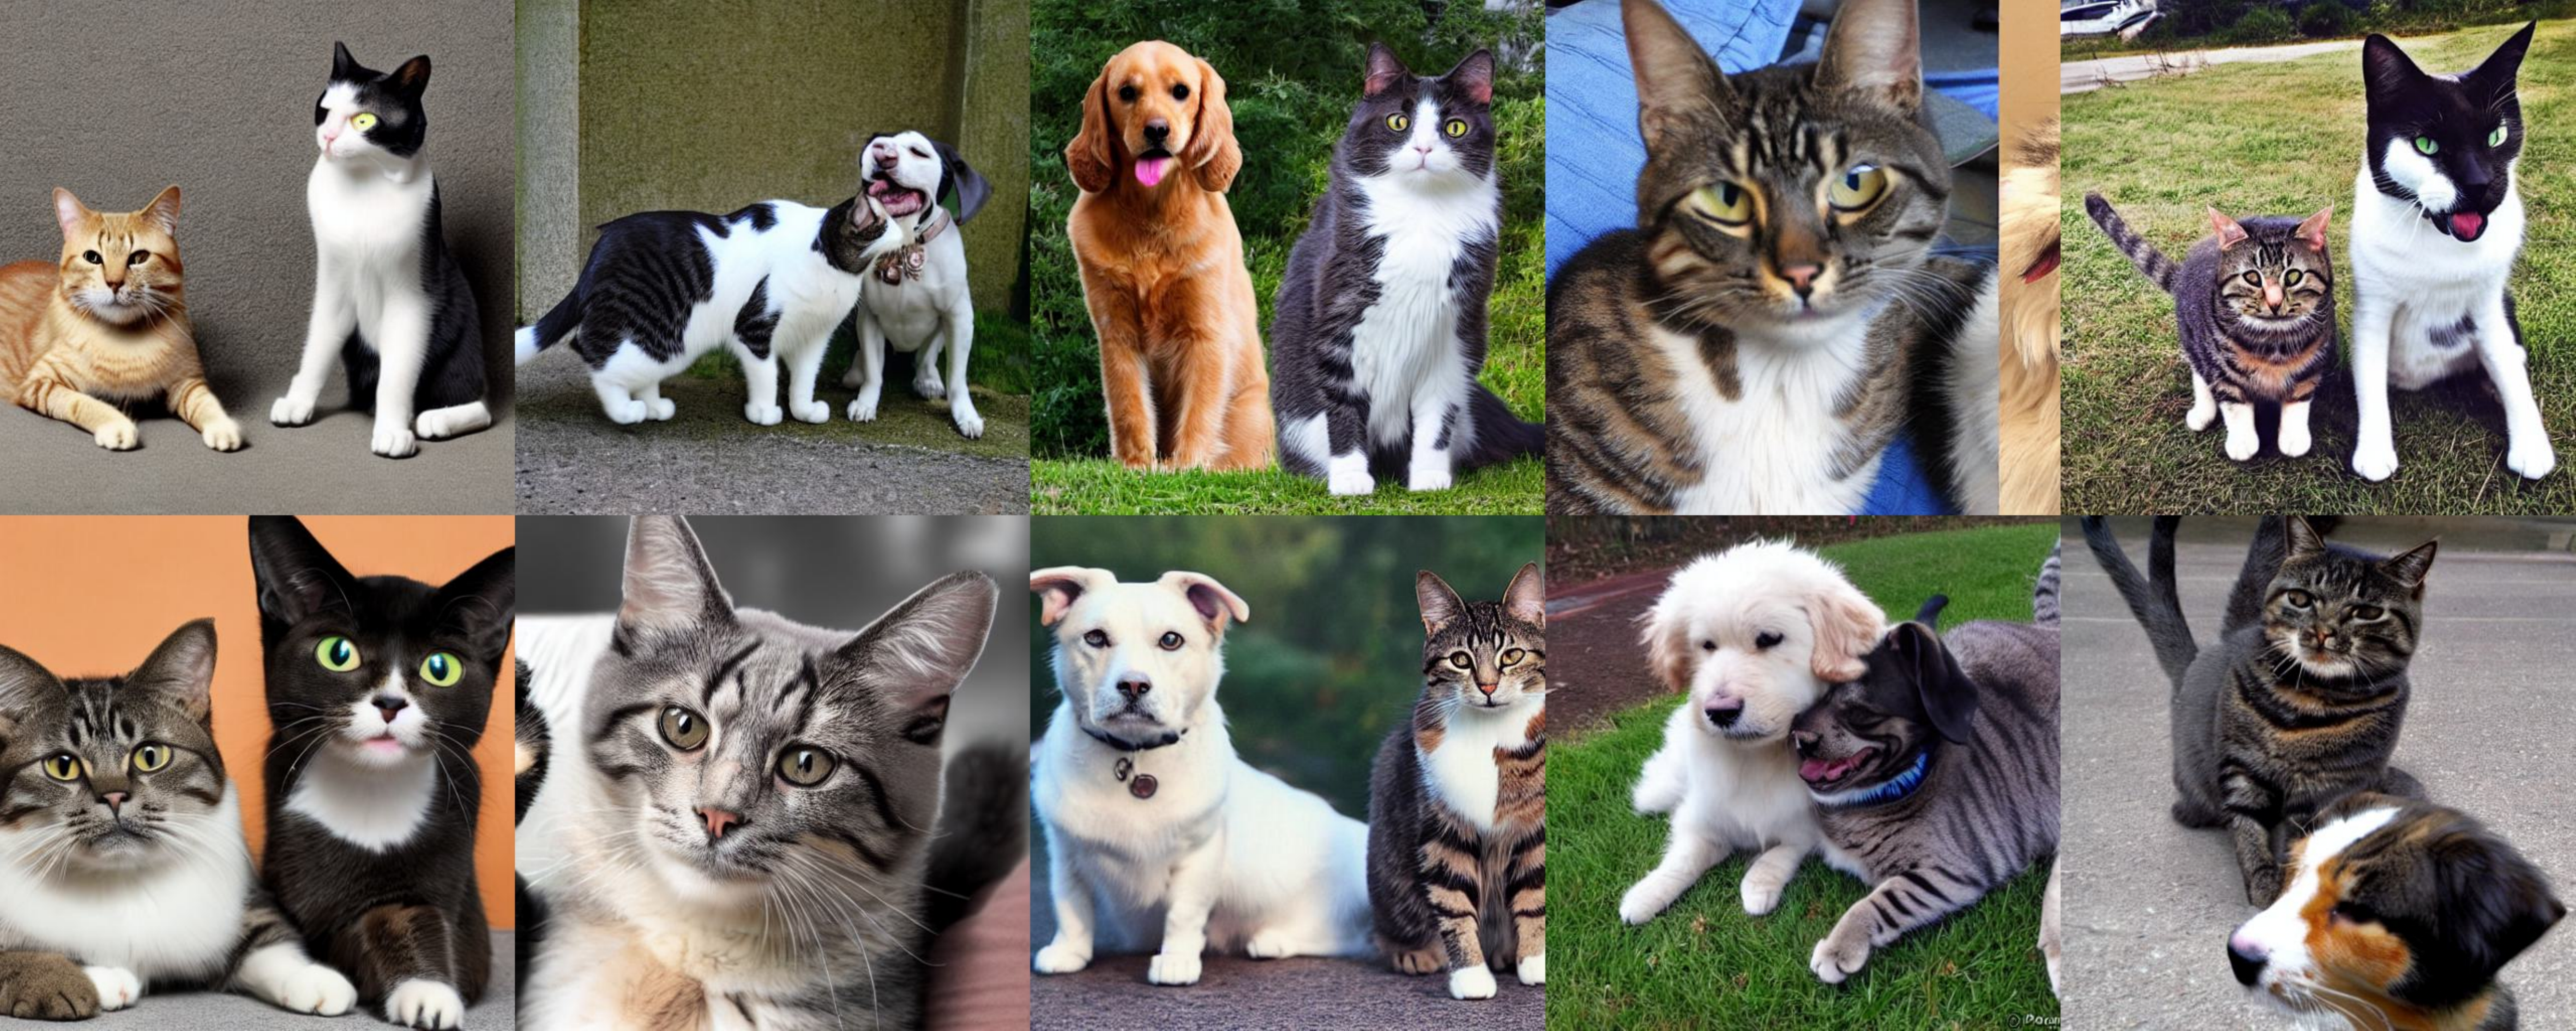}
\label{fig:app_comp_0}} 
\subfigure[SFT model]
{\includegraphics[width=0.99\textwidth]{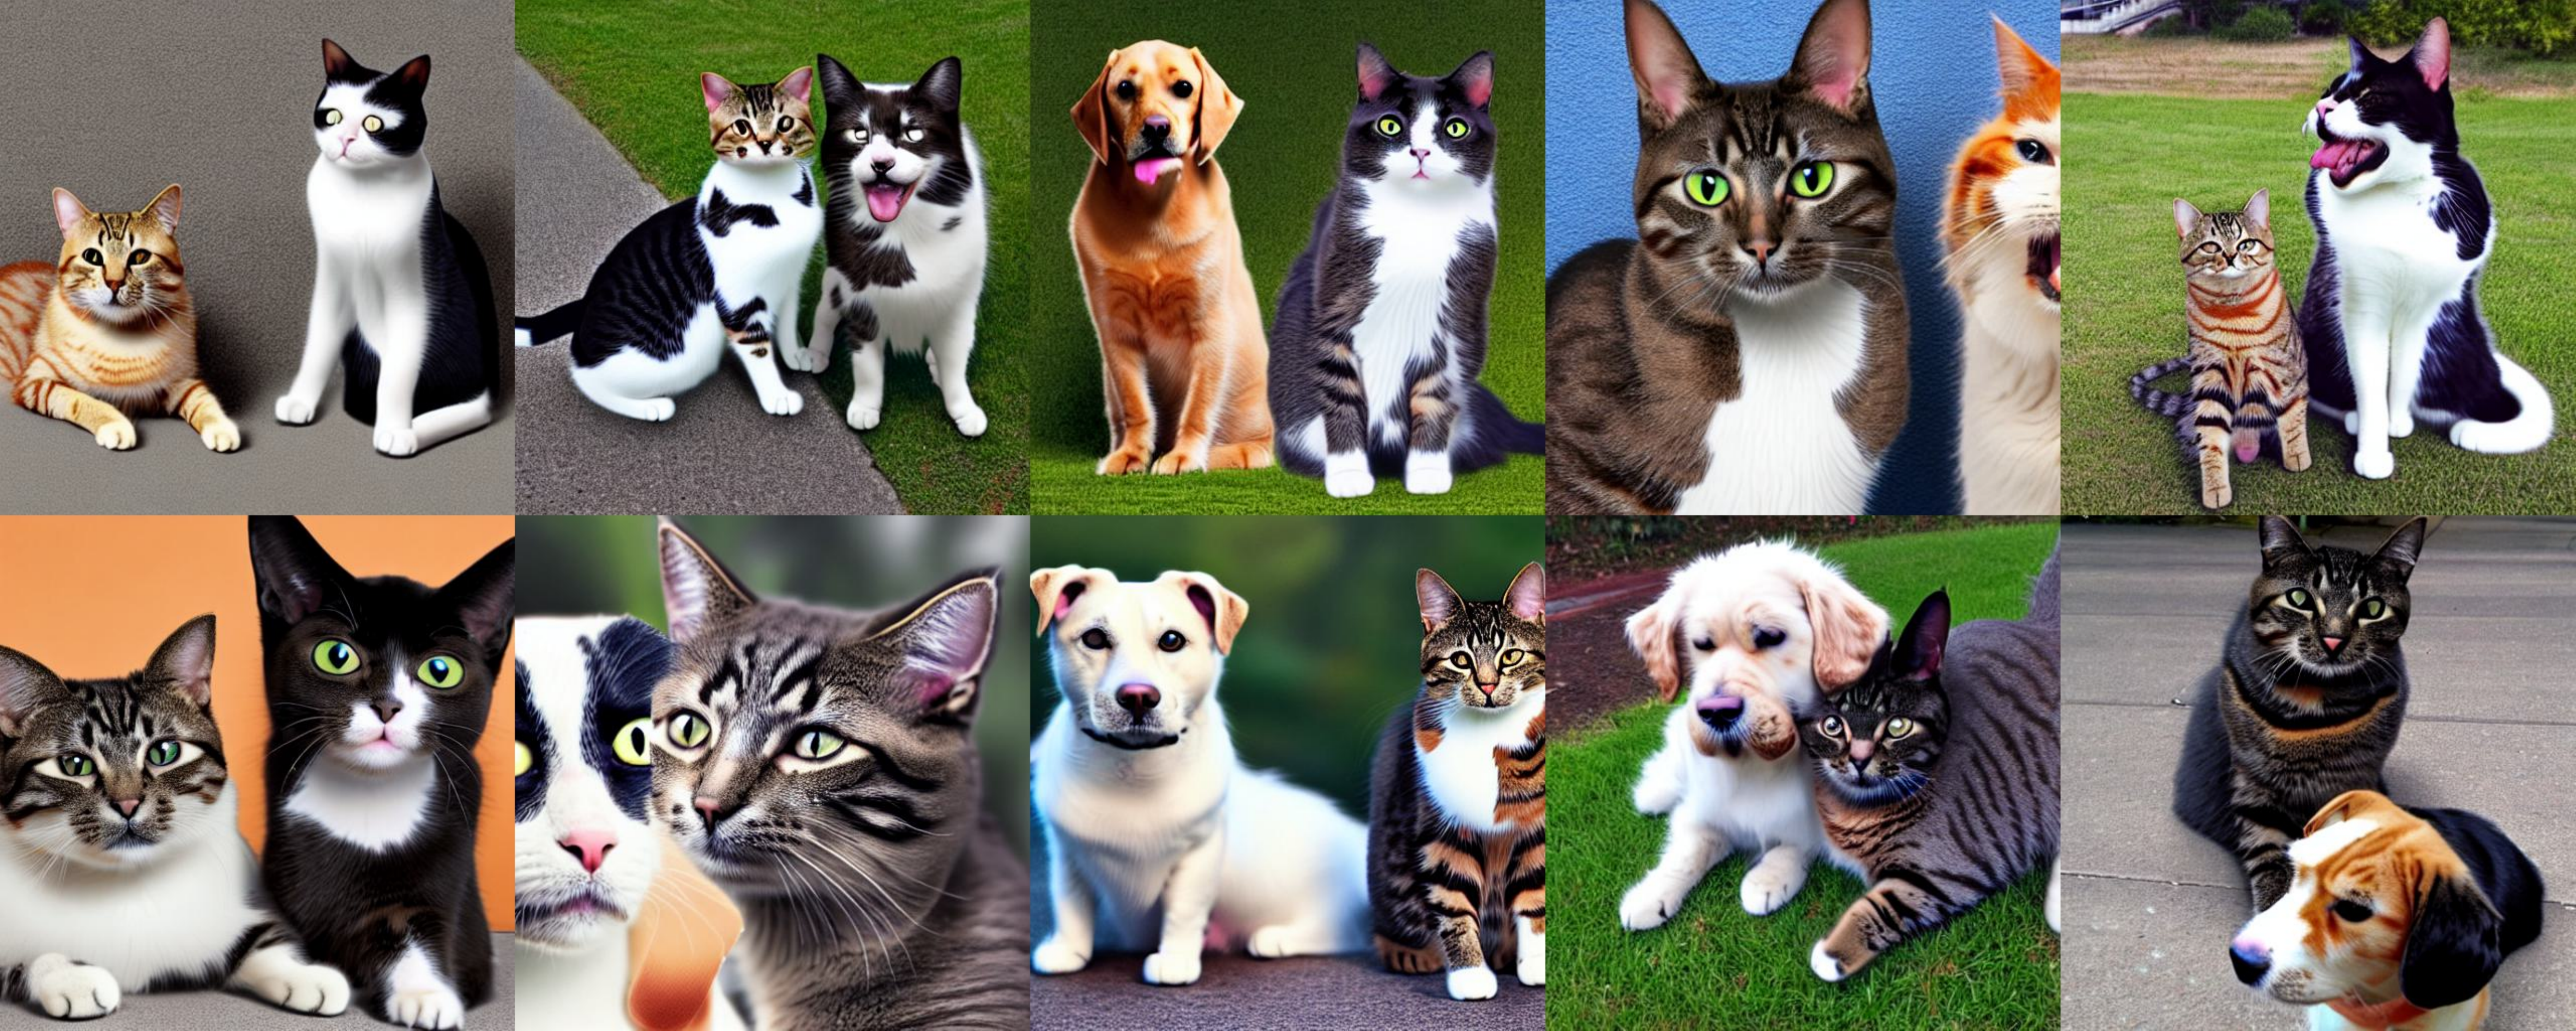}
\label{fig:app_comp_1}}
\subfigure[RL model]
{\includegraphics[width=0.99\textwidth]{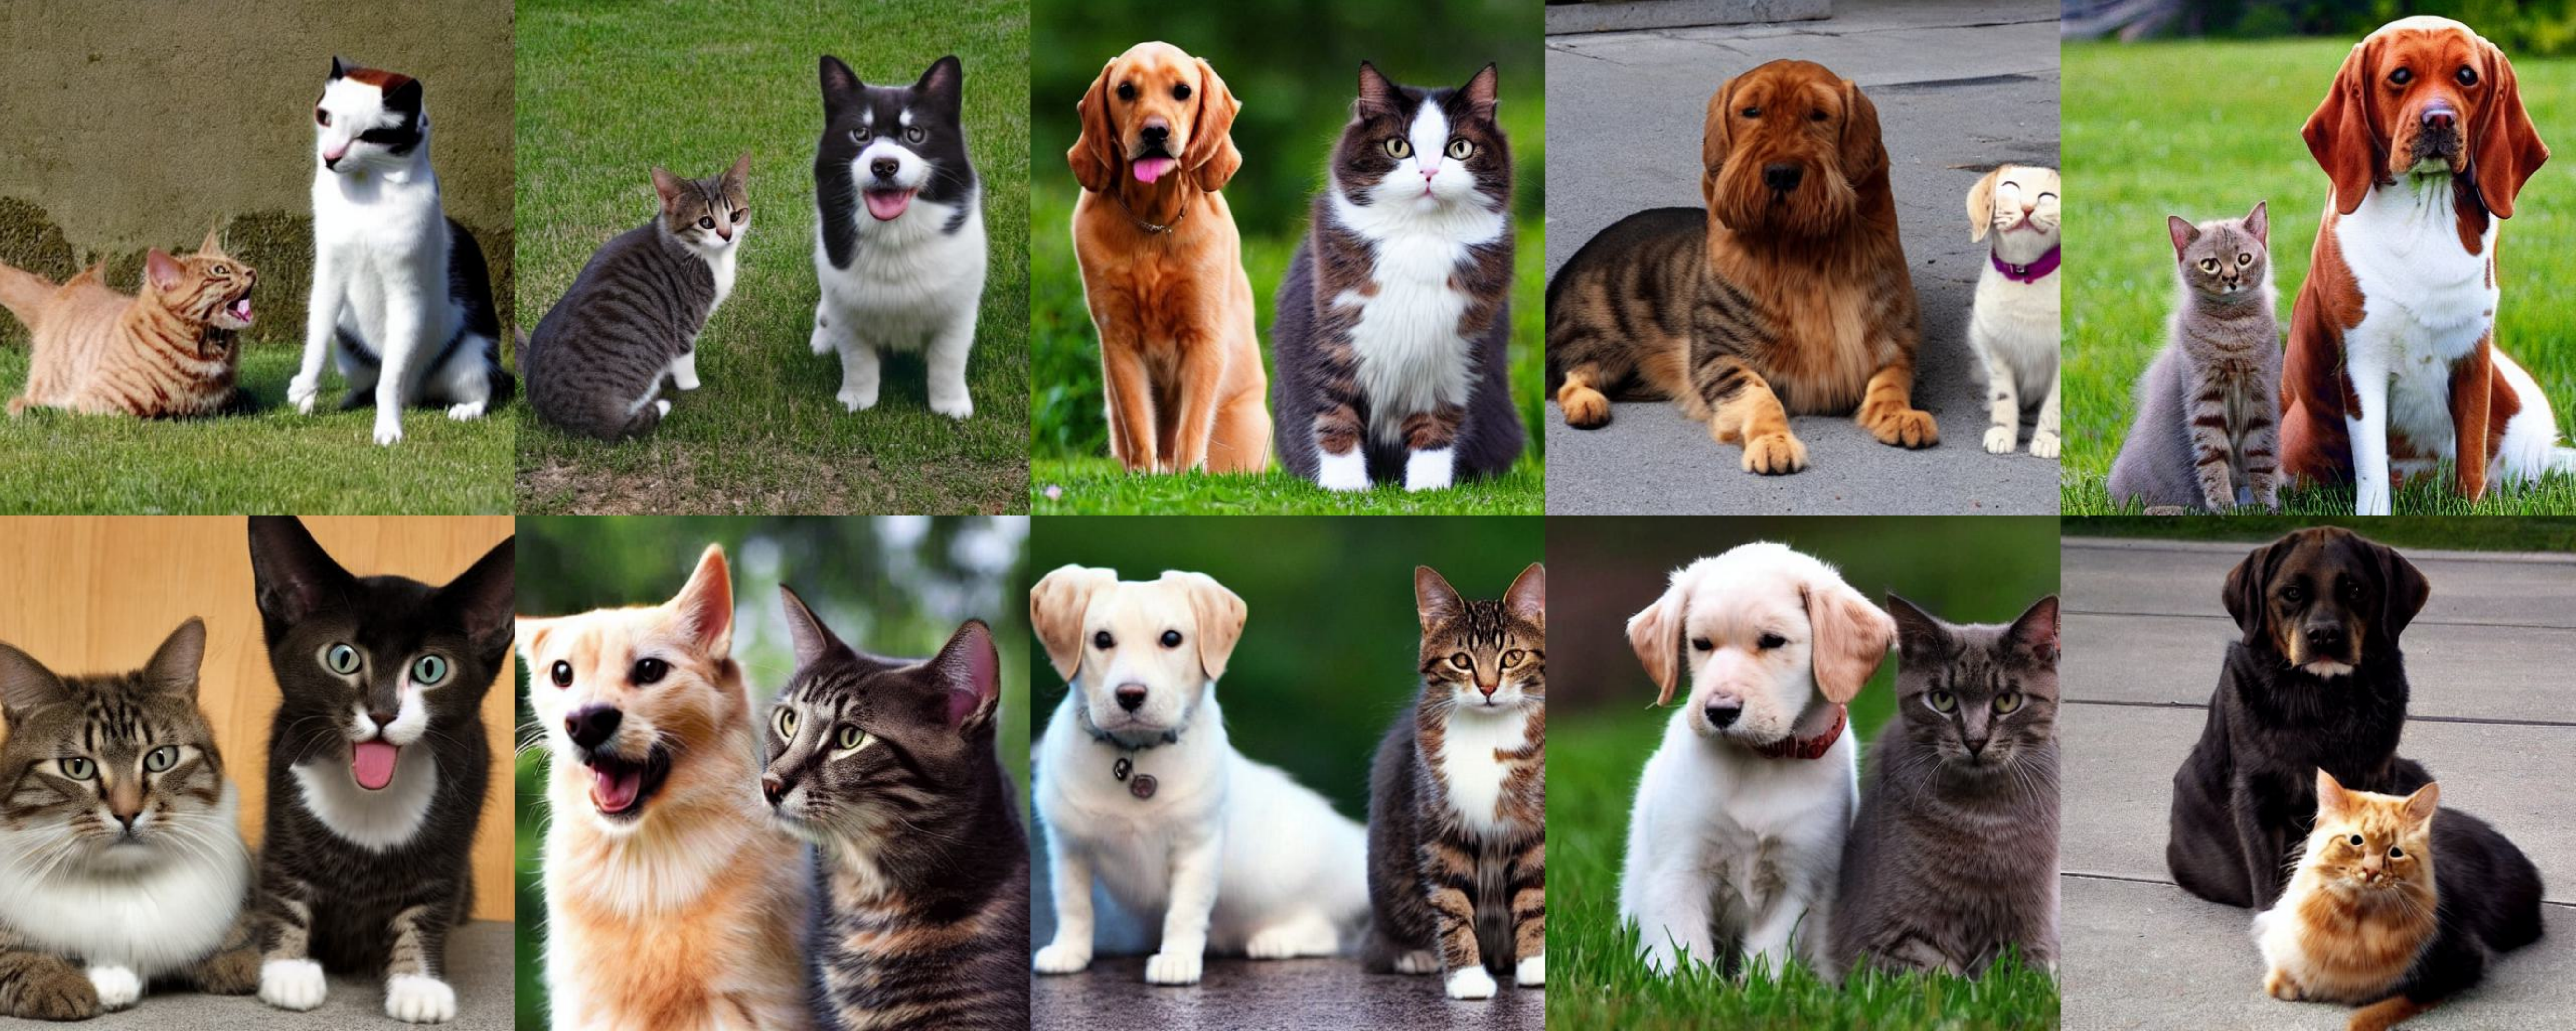}
\label{fig:app_comp_2}}
\caption{Non-cherry-picked samples from (a) the original Stable Diffusion model, (b) supervised fine-tuned (SFT) model and (c) RL fine-tuned model.}
\label{fig:app_comp}
\end{figure*}

\begin{figure*} [h!] \centering
\subfigure[Original model]
{\includegraphics[width=0.99\textwidth]{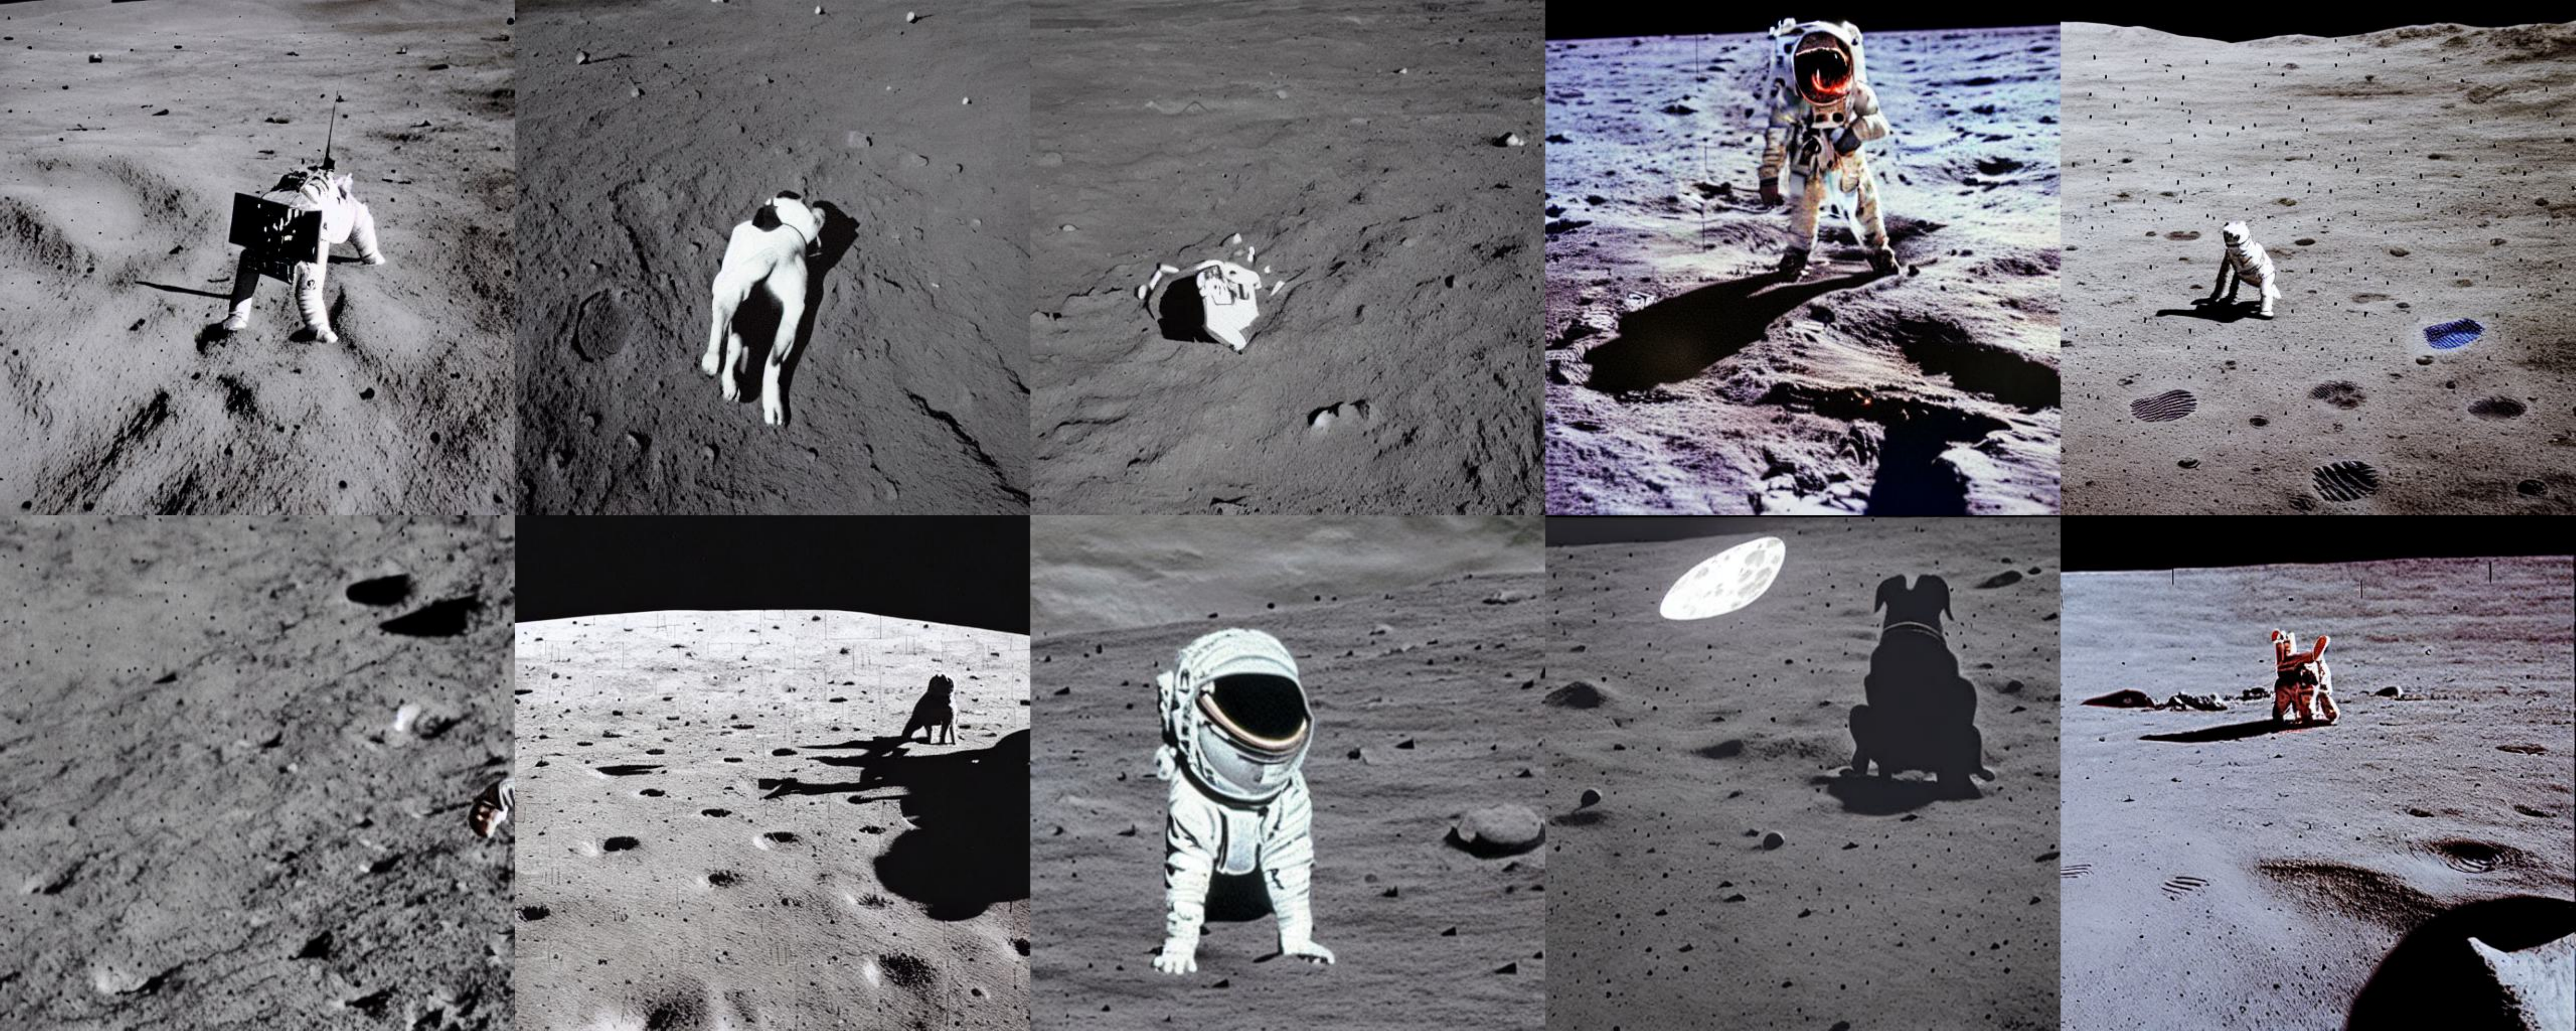}
\label{fig:app_loc_0}} 
\subfigure[SFT model]
{\includegraphics[width=0.99\textwidth]{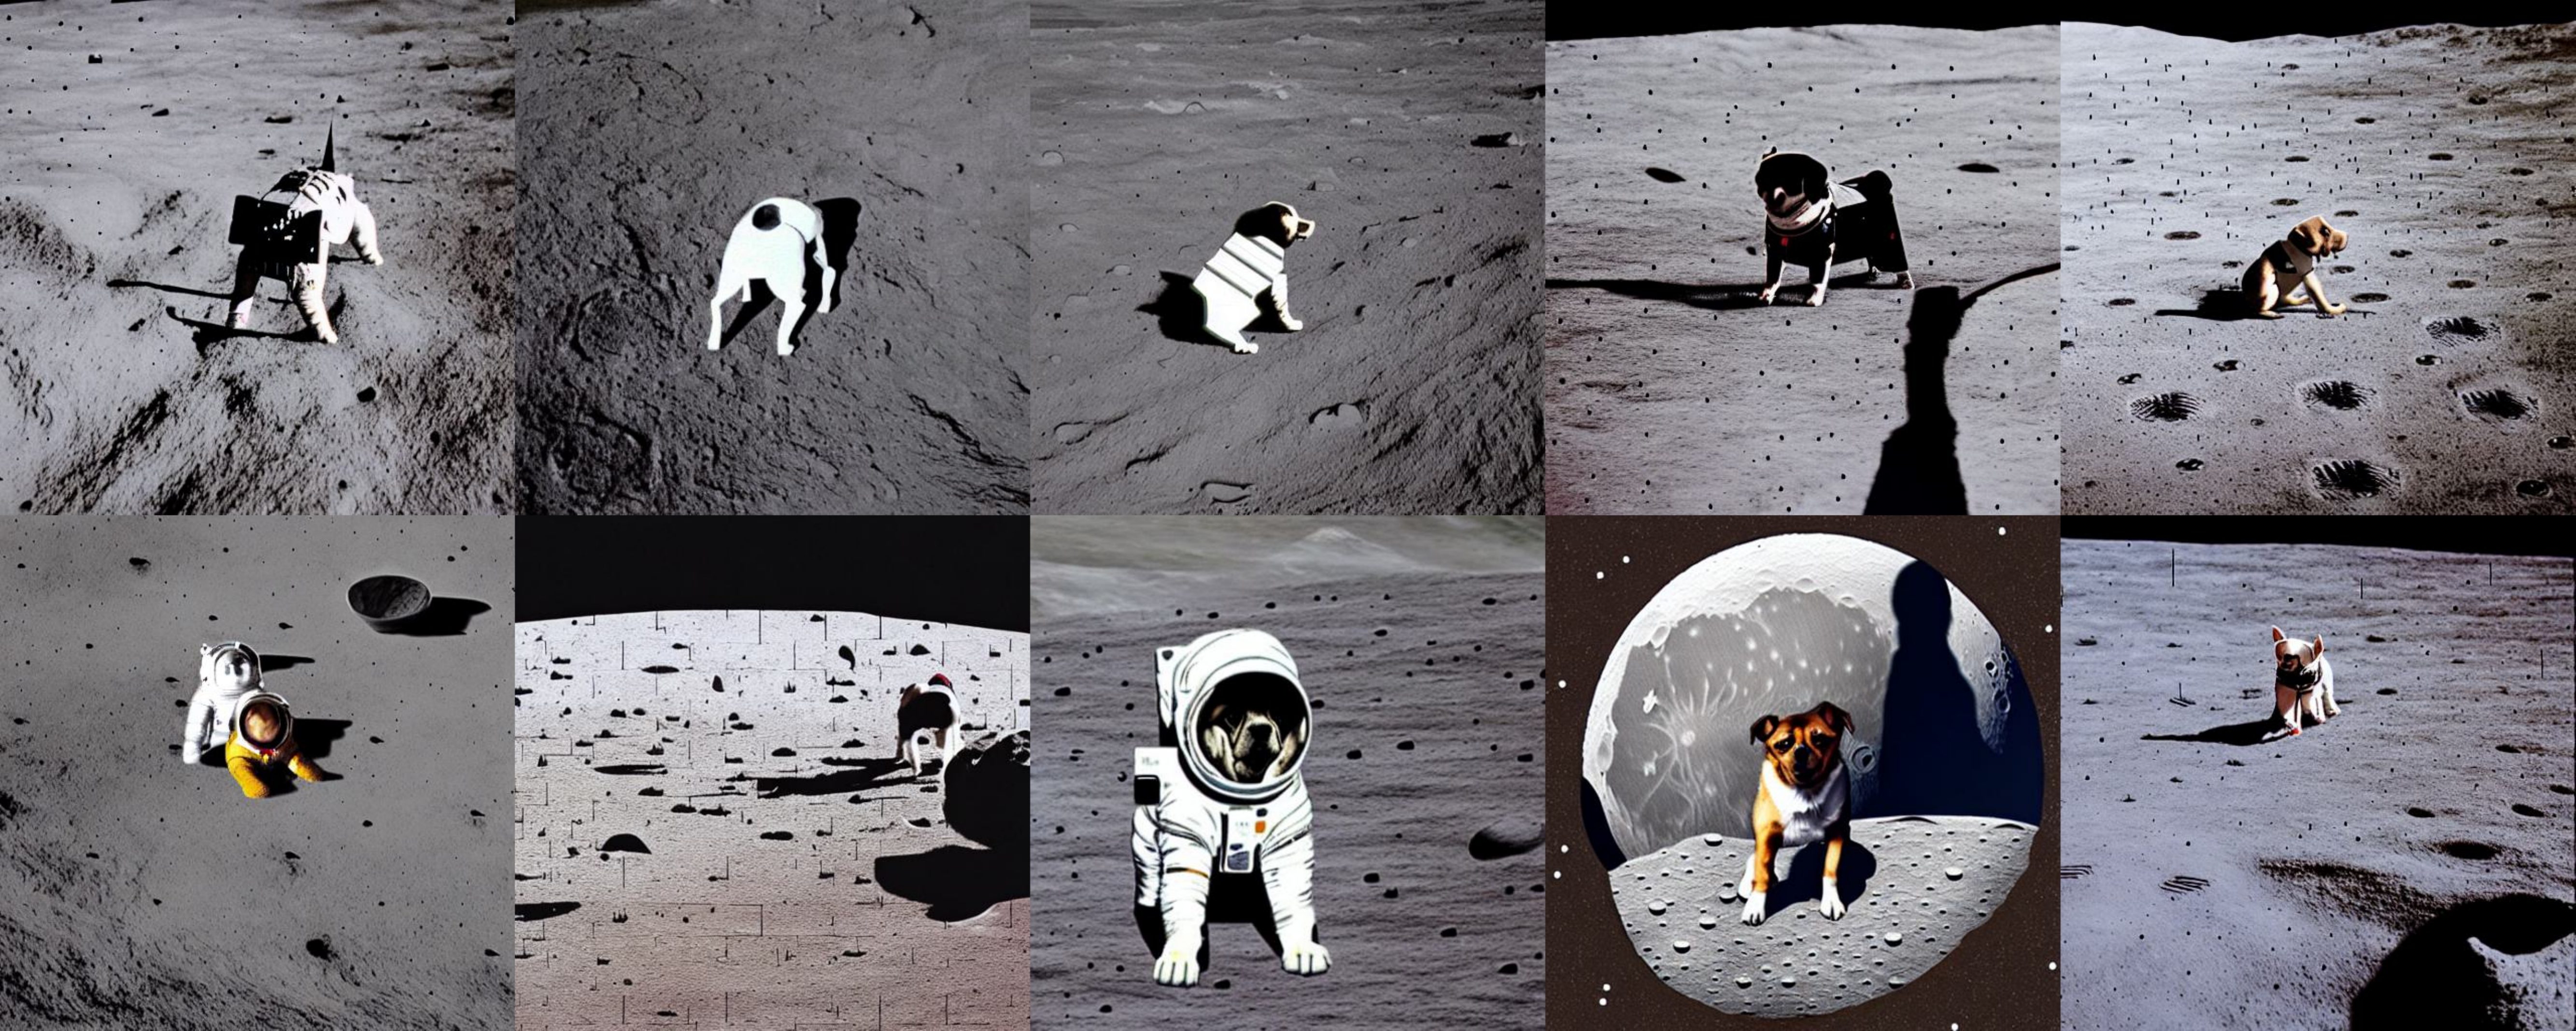}
\label{fig:app_loc_1}}
\subfigure[RL model]
{\includegraphics[width=0.99\textwidth]{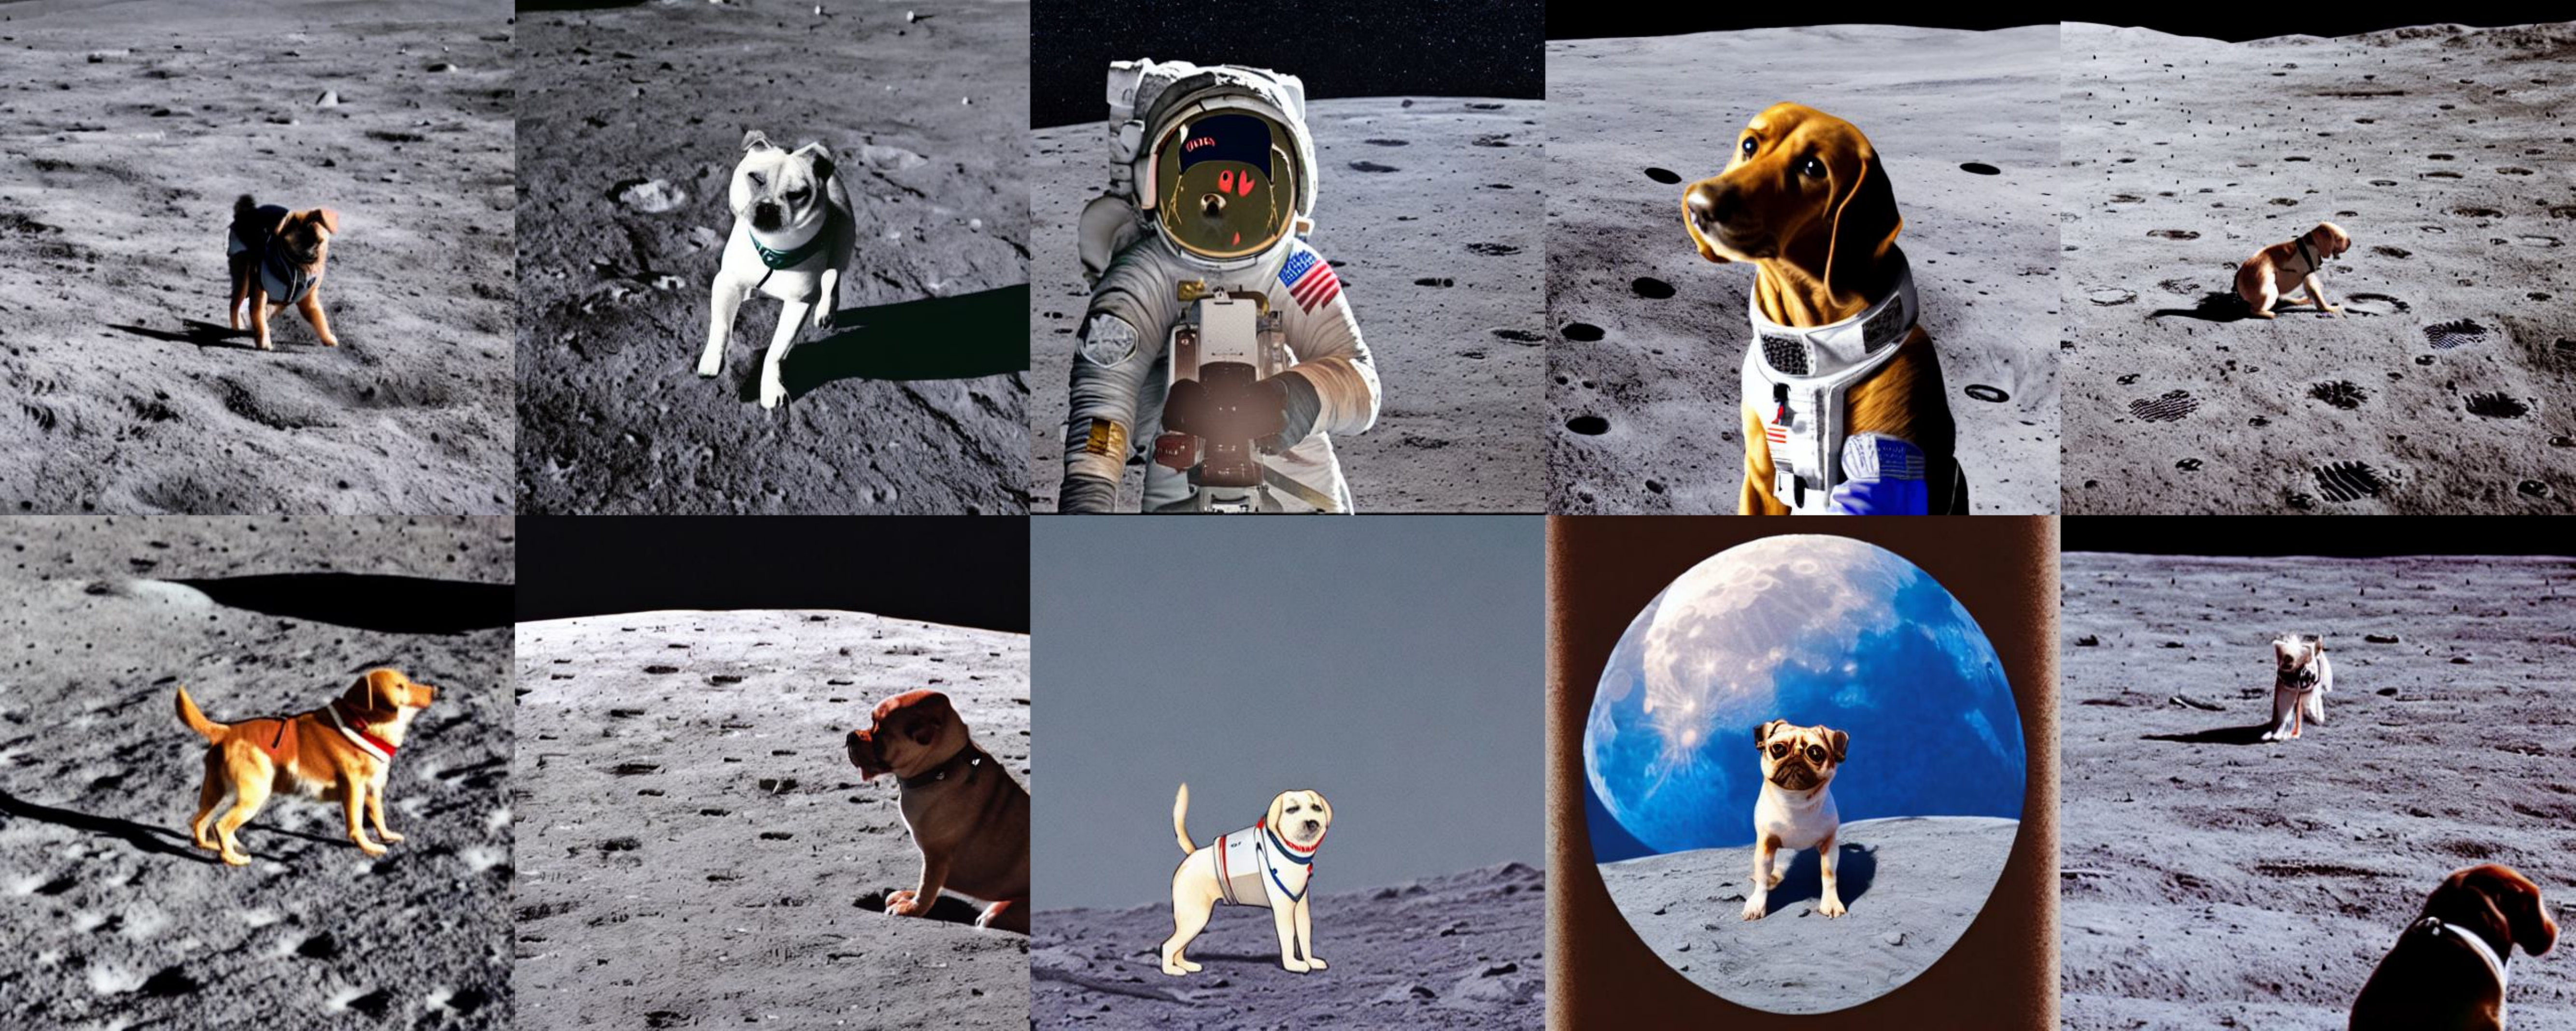}
\label{fig:app_loc_2}}
\caption{Non-cherry-picked samples from (a) the original Stable Diffusion model, (b) supervised fine-tuned (SFT) model and (c) RL fine-tuned model.}
\label{fig:app_loc}
\end{figure*}

\begin{figure*} [h!] \centering
\subfigure[RL model without KL regularization]
{\includegraphics[width=0.99\textwidth]{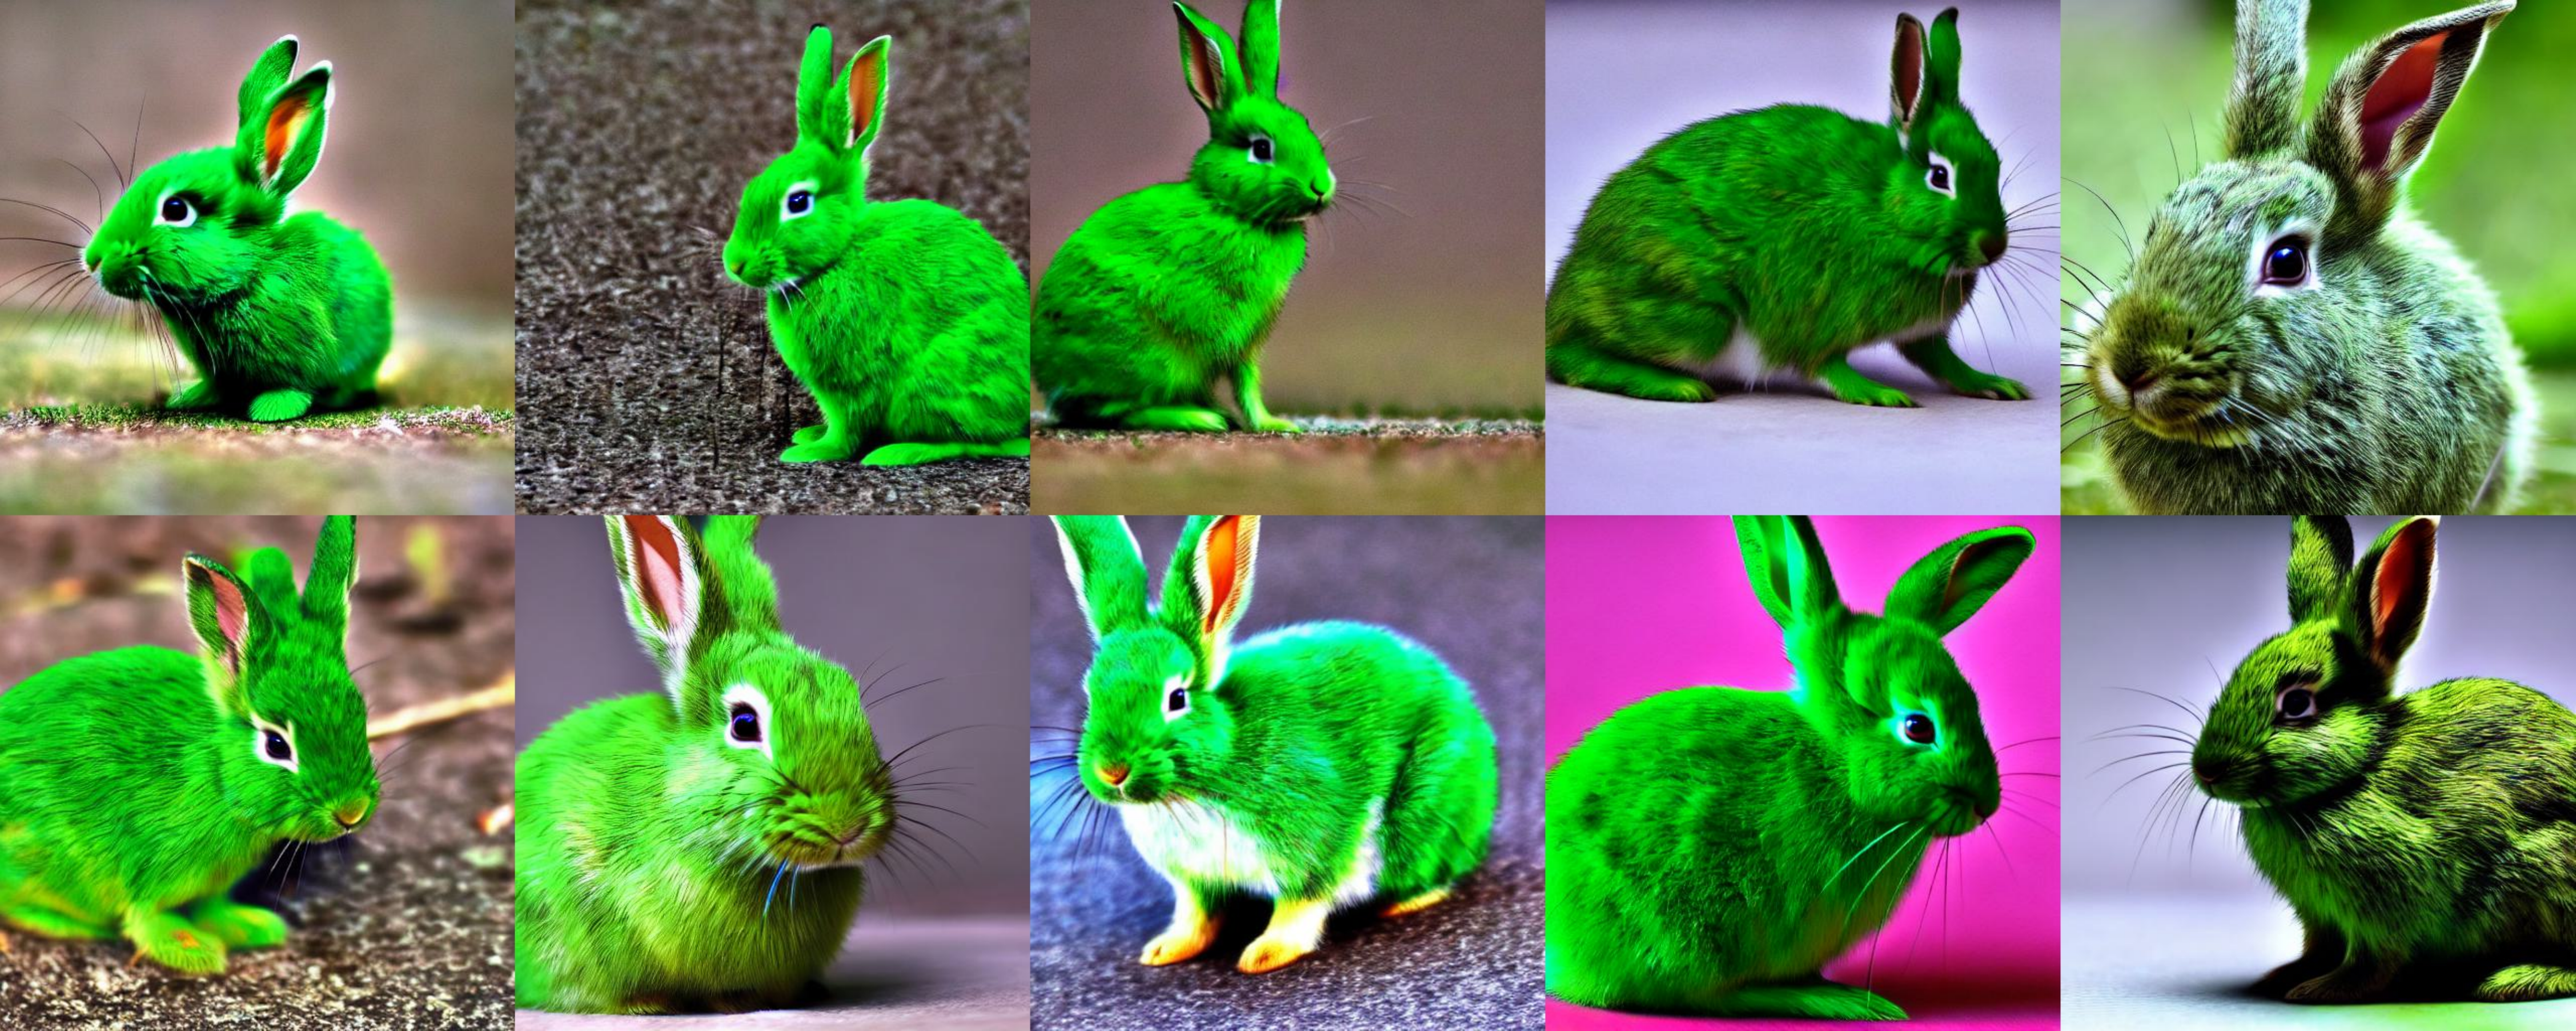}
\label{fig:app_kl_rl_kl}} 
\subfigure[RL model with KL regularization]
{\includegraphics[width=0.99\textwidth]{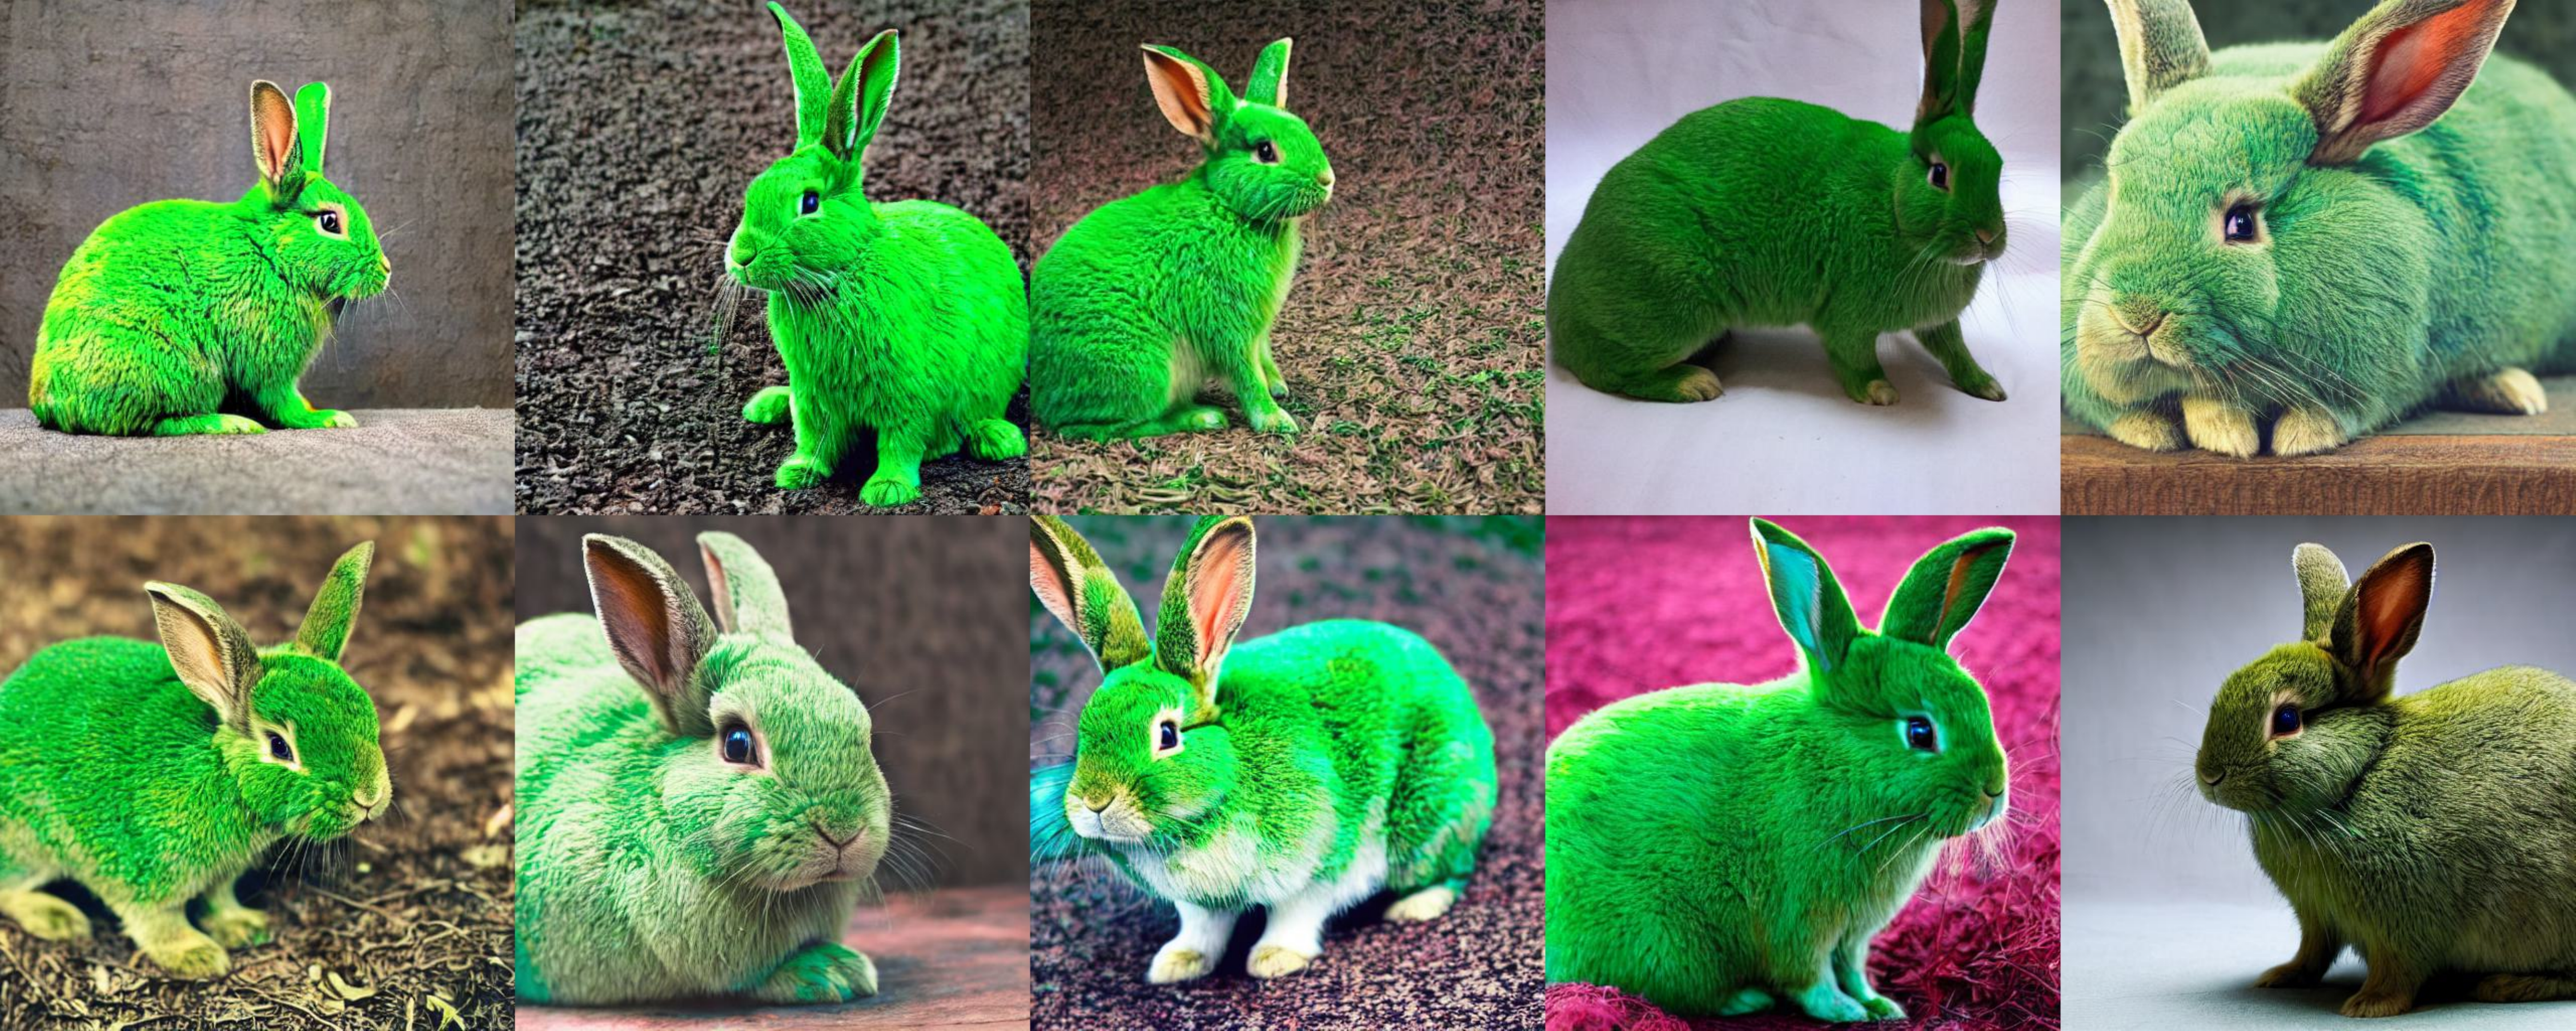}
\label{fig:app_kl_rl_no_kl}}
\caption{Non-cherry-picked samples from RL fine-tuned models (a) without and (b) with KL regularization.}
\label{fig:app_kl_rl}
\end{figure*}

\begin{figure*} [h!] \centering
\subfigure[SFT model without KL regularization]
{\includegraphics[width=0.99\textwidth]{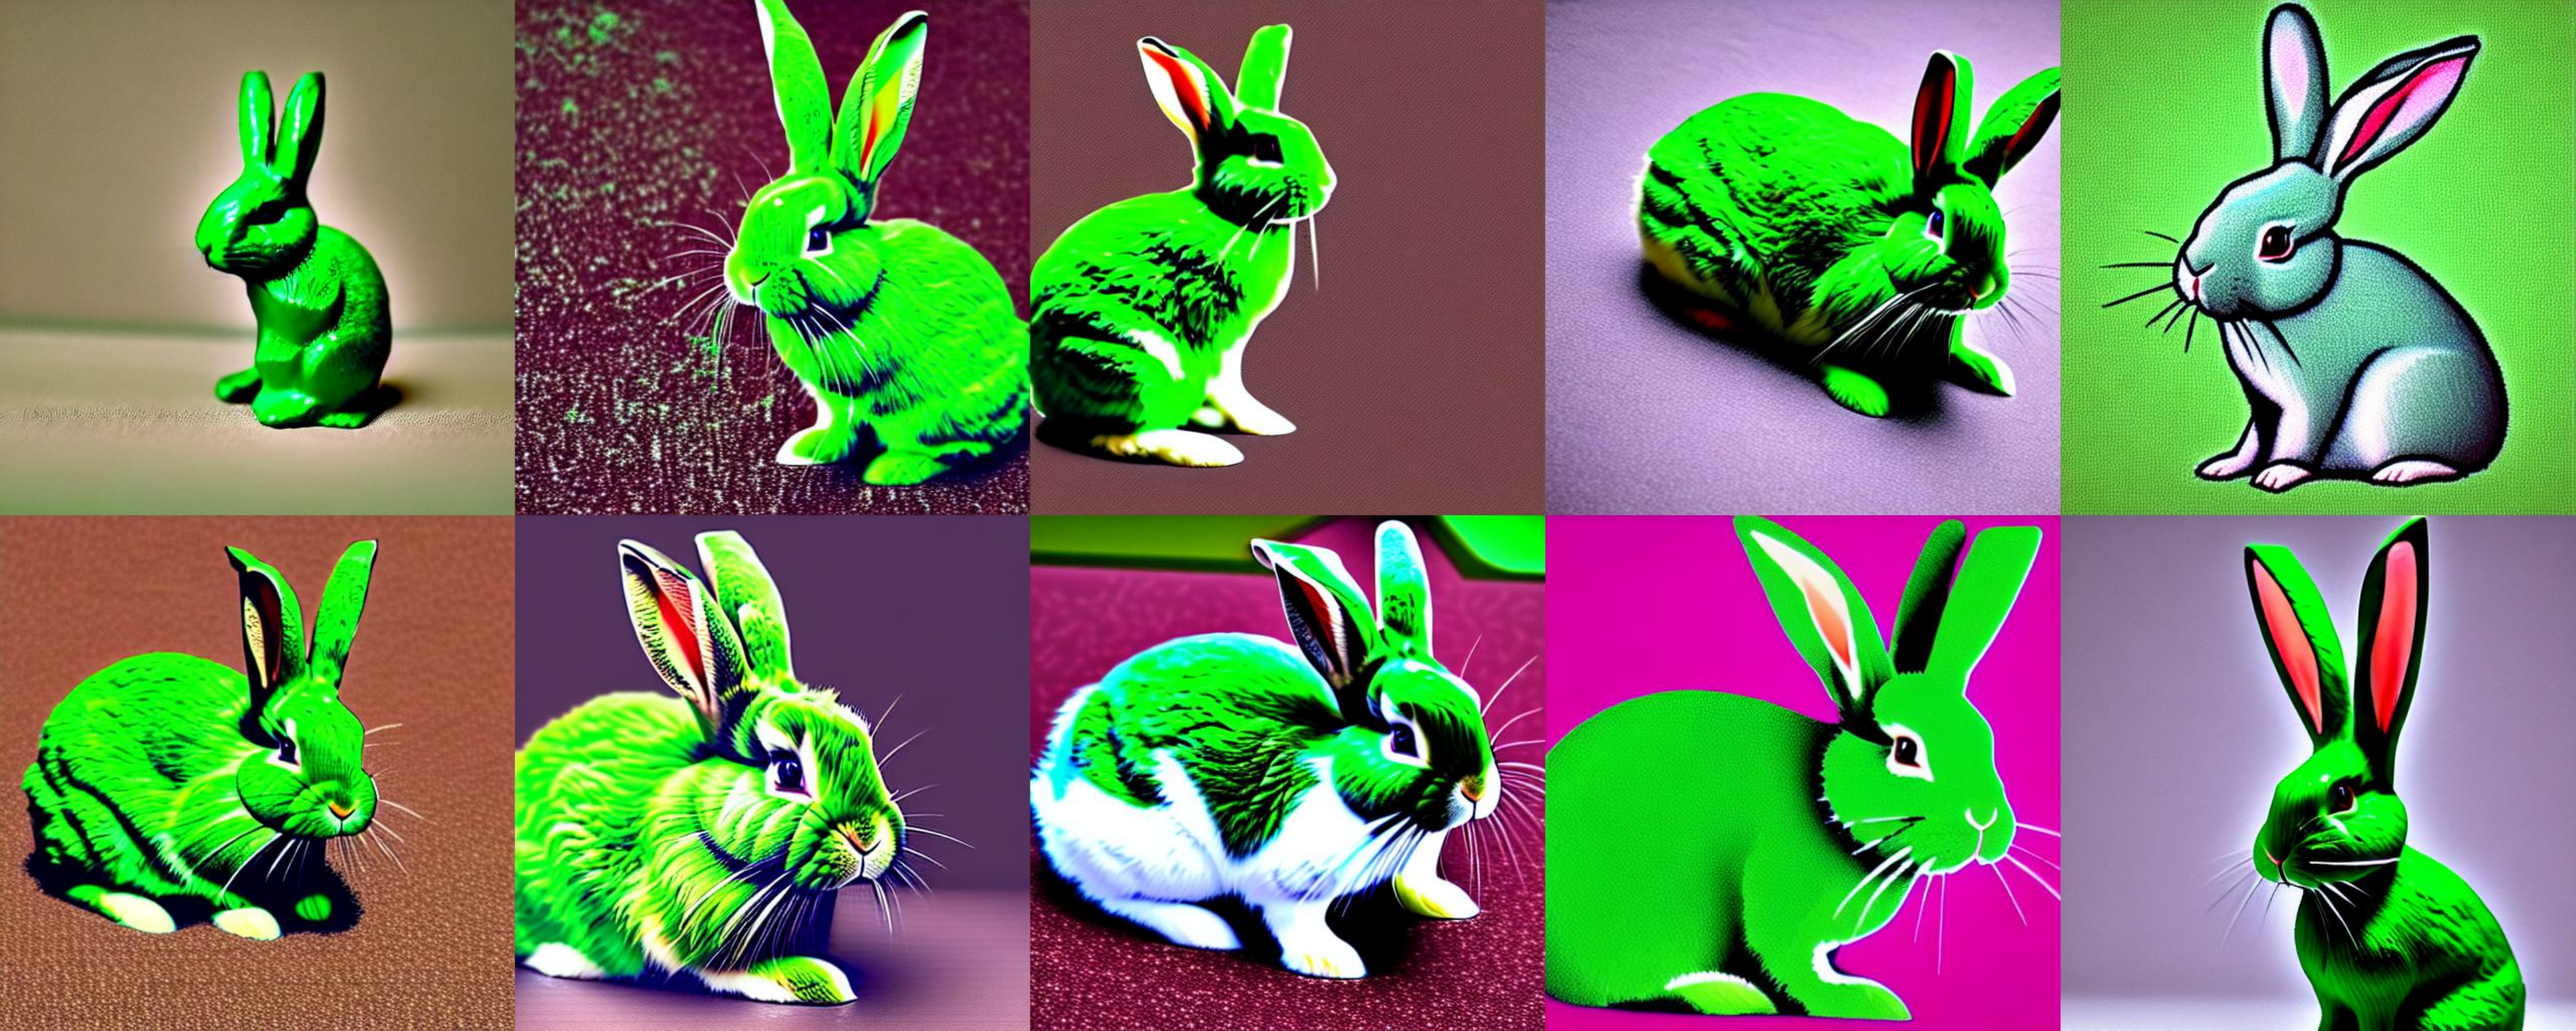}
\label{fig:app_kl_sup_kl}} 
\subfigure[SFT model with KL regularization]
{\includegraphics[width=0.99\textwidth]{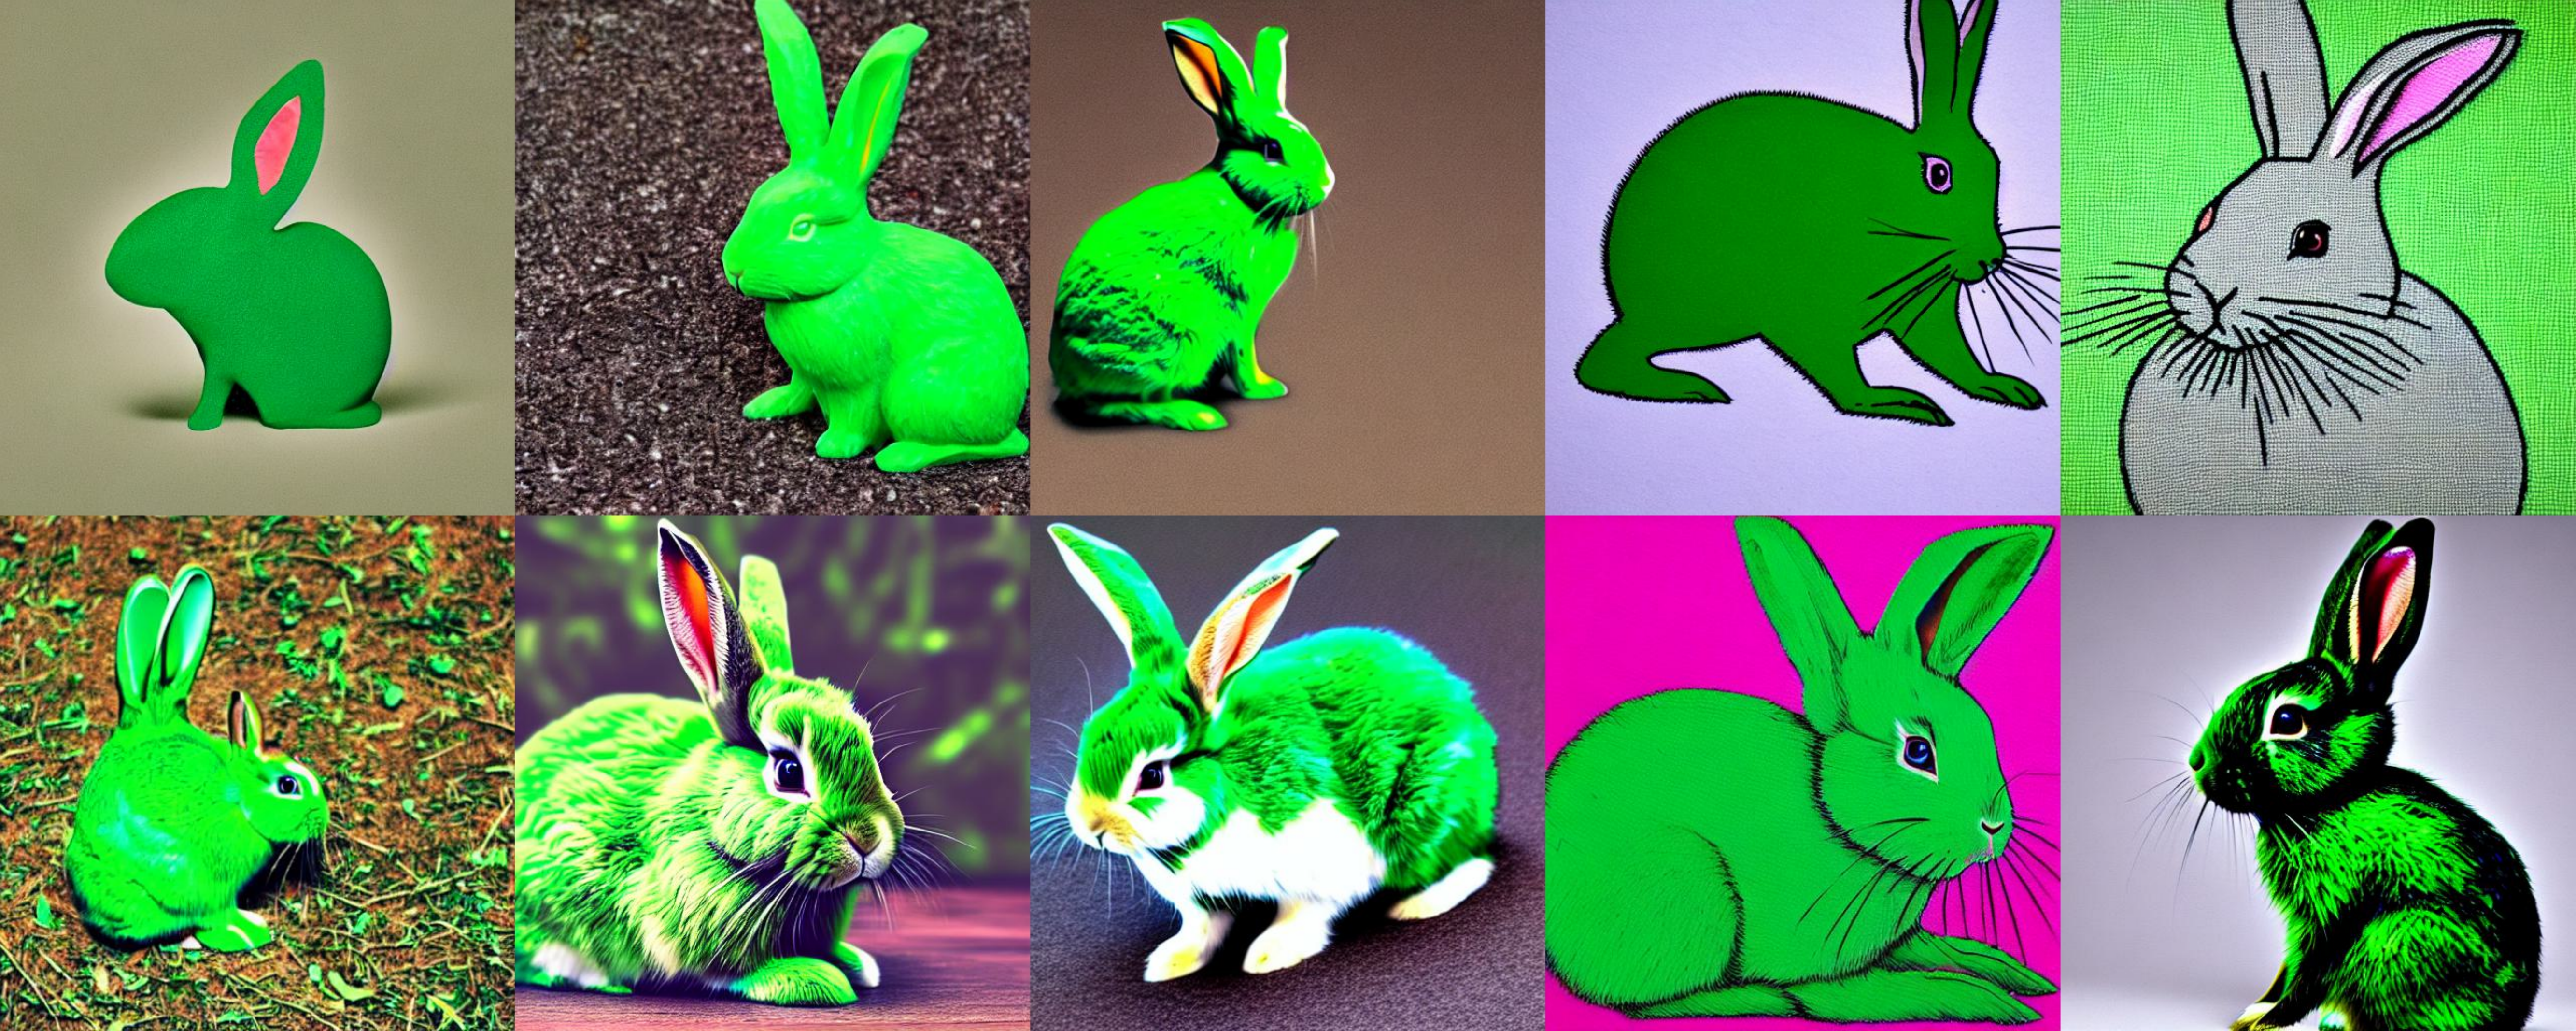}
\label{fig:app_kl_sup_no_kl}}
\caption{Non-cherry-picked samples from supervised fine-tuned (SFT) models (a) without and (b) with KL regularization.}
\label{fig:app_kl_sup}
\end{figure*}
